# Supplementary material for: Rethinking Graph Neural Networks for the Graph Coloring Problem
Source: arXiv:2208.06975 source file (2022-08-19)
Supplement: Supplementary file 2 [file Appendix.pdf]

# Appendix: Rethinking Graph Neural Networks for the Graph Coloring Problem

## Graph Terminology

Here we list the following graph theoretic terms encountered in our work. Let  $\mathcal{G} = (\mathcal{V}, \mathcal{E})$  and  $\mathcal{G}' = (\mathcal{V}', \mathcal{E}')$  be graphs on vertex set  $\mathcal{V}$  and  $\mathcal{V}'$ , we define

- *isomorphism*: we say that a bijection  $\pi : \mathcal{V} \rightarrow \mathcal{V}'$  is an *isomorphism* if any two vertices  $u, v \in \mathcal{V}$  are adjacent in  $\mathcal{G}$  if and only if  $\pi(u), \pi(v) \in \mathcal{V}'$  are adjacent in  $\mathcal{G}'$ , i.e.,  $\{u, v\} \in \mathcal{E}$  iff  $\{\pi(u), \pi(v)\} \in \mathcal{E}'$ .
- *isomorphic nodes*: If there exists the isomorphism between  $\mathcal{G}$  and  $\mathcal{G}'$ , we say that  $\mathcal{G}$  and  $\mathcal{G}'$  are *isomorphic*.
- *automorphism*: When  $\pi$  is an isomorphism of a vertex set onto itself, i.e.,  $\mathcal{V} = \mathcal{V}'$ ,  $\pi$  is called an *automorphism* of  $\mathcal{G}$ .
- *topologically equivalent*: We say that the node pair  $\{u, v\}$  is *topologically equivalent* if there is an automorphism mapping one to the other, i.e.,  $v = \pi(u)$ .
- *equivalent*:  $\{u, v\}$  is *equivalent* if it is topologically equivalent by  $\pi$  and  $\mathbf{x}_w = \mathbf{x}_{\pi(w)}$  holds for every  $w \in \mathcal{V}$ , where  $\mathbf{x}_w$  is the node attribute of node  $w$ .
- *r-local equivalent*:  $\{u, v\}$  is *r-local equivalent* if it is *r*-local topologically equivalent by  $\pi_r$  and  $\mathbf{x}_w = \mathbf{x}_{\pi_r(w)}$  holds for every  $w \in \mathcal{B}_{\mathcal{G}}(u, r)$ .
- *r-local isomorphism*: A bijection  $\pi_r$  is an *r-local isomorphism* that maps  $u$  to  $v$  if  $\pi_r$  is an isomorphism that maps  $\mathcal{B}_{\mathcal{G}}(u, r)$  to  $\mathcal{B}_{\mathcal{G}}(v, r)$ .

## Proofs

### Proof of Property 1

We first recall the property.

**Property 1.** All AC-GNNs cannot discriminate any equivalent node pair.

*Proof.* Let  $\pi$  be the automorphism mapping  $u$  to  $v$ , here, we propose a stronger property:

**Property 1.** Given an AC-GNN and an equivalent node pair  $\{u, v\}$  by  $\pi$ ,  $\mathbf{h}_w^i = \mathbf{h}_{\pi(w)}^i$  holds for any iteration  $i$  and any node  $w \in \mathcal{V}$ .

Copyright © 2022, Association for the Advancement of Artificial Intelligence (www.aaai.org). All rights reserved.

This apparently holds for  $i = 0$  since  $\mathbf{x}_w = \mathbf{x}_{\pi(w)}$ ,  $\forall w \in \mathcal{V}$ . Suppose this holds for iteration  $j$ , i.e.,  $\mathbf{h}_w^j = \mathbf{h}_{\pi(w)}^j$ ,  $\forall w \in \mathcal{V}$ . By definition, AC-GNN  $\mathcal{A}$  produces the feature vector  $\mathbf{h}_v^{j+1}$  of node  $v$  in the  $(j + 1)_{th}$  iteration as follows:

$$\mathbf{h}_v^{(j+1)} = \text{COM}^{(j+1)}(\mathbf{h}_v^{(j)}, \text{AGG}^{(j+1)}(\{\mathbf{h}_u^{(j)} : u \in \mathcal{N}(v)\})). \quad (1)$$

Since an automorphism  $\pi$  remains the set of edges, i.e.,  $\{u, v\} \in \mathcal{E}$  iff  $\{\pi(u), \pi(v)\} \in \mathcal{E}$ , the connection relation between two neighbors is preserved after the permutation by  $\pi$ , that is,  $\mathcal{N}(\pi(v)) = \{\pi(u), u \in \mathcal{N}(v)\}$  for any  $v \in \mathcal{V}$ . Then, the input of  $\text{AGG}^{(j+1)}$  for  $\pi(v)$  is given by  $\{\mathbf{h}_u^{(j)} : u \in \mathcal{N}(\pi(v))\}$ , which is  $\{\mathbf{h}_{\pi(u)}^{(j)} : u \in \mathcal{N}(v)\}$ . Since  $\mathbf{h}_w^j = \mathbf{h}_{\pi(w)}^j$ ,  $\forall w \in \mathcal{V}$ , the input of  $\text{AGG}^{(j+1)}$  for  $v$  is equal to the one of  $\text{AGG}^{(j+1)}$  for  $\pi(v)$ , i.e.,  $\{\mathbf{h}_{\pi(u)}^{(j)} : u \in \mathcal{N}(v)\} = \{\mathbf{h}_u^{(j)} : u \in \mathcal{N}(v)\}$  and makes their output equal, i.e.,  $\mathbf{m}_v^{j+1} = \mathbf{m}_{\pi(v)}^{j+1}$ . Therefore, the input of  $\text{COM}^{(j+1)}$  for  $v$ ,  $(\mathbf{h}_v^{(j)}, \mathbf{m}_v^{j+1})$ , is also equal to the one of  $\text{COM}^{(j+1)}$  for  $\pi(v)$ , which makes the vector features of  $v$  and  $\pi(v)$  equal after  $(j + 1)_{th}$  iteration for any node  $v \in \mathcal{V}$  and proves the property 1. Thus, the AC-GNN  $\mathcal{A}$  always produces the same node embeddings for the nodes in the equivalent node pair, which results in the same color.  $\square$

### Proof of Property 2

We first recall the property.

**Property 2.** If a graph  $\mathcal{G}$  contains two connected nodes  $u$  and  $v$  that share the same neighborhood except each other, i.e.,  $\mathcal{N}(u) \setminus \{v\} = \mathcal{N}(v) \setminus \{u\}$ , then an integrated AC-GNN cannot discriminate  $\{u, v\}$ .

*Proof.* The proof starts with a simple fact: a classifier  $\text{CLS}(\cdot)$  always assigns two nodes with the same node embedding to the same category. It follows that the inputs for the node features of  $u$  and  $v$  after iteration  $k$  are exactly the same since  $\mathcal{N}(u) \cup \{u\} = \mathcal{N}(u) \setminus \{v\} \cup \{u, v\} = \mathcal{N}(v) \setminus \{u\} \cup \{u, v\} = \mathcal{N}(v) \cup \{v\}$ . Therefore, the outputs are the same, which means that  $\mathbf{h}_u^{(j)} = \mathbf{h}_v^{(j)}$  holds for any iteration  $k$  and any aggregation and combine functions  $\text{AGG}(\cdot)$ ,  $\text{COM}(\cdot)$ . Combining with the fact

that  $CLS(\mathbf{h}_u) = CLS(\mathbf{h}_v)$  if  $\mathbf{h}_u = \mathbf{h}_v$ , the proof is finished.  $\square$

### Proof of Corollary 1

We first recall the corollary.

**Corollary 1.** *A local coloring method is non-optimal in the random  $d$ -regular graph as  $d \rightarrow \infty$ .*

*Proof.* A random  $d$ -regular graph  $\mathcal{G}_d^n$  is a graph with  $n$  nodes and each node pair is connected with a probability  $d/n$ . We start the proof from the following non-trivial property:

**Property 2** ((Rahman, Virag et al. 2017)). *The largest density of factor of i.i.d. independent sets in a random  $d$ -regular graph is asymptotically at most  $(\log d)/d$  as  $d \rightarrow \infty$ . The density of the largest independent sets in these graphs is asymptotically  $2(\log d)/d$ .*

The property above limits the size of an independent set produced by local method for the random  $d$ -regular graph with an upper bound,  $n(\log d)/d$  as  $d \rightarrow \infty$ . Given an upper bound of the independent set, the following corollary on the graph coloring problem is introduced:

**Corollary 3.** *The lower bound of  $k$  with a zero conflict constraint obtained by a local coloring method for the random  $d$ -regular graph is  $d/\log d$  as  $d \rightarrow \infty$ .*

The proof is based on the Property 2: if a local coloring method  $f$  obtains a smaller  $k'$ , s.t.  $k' < d/\log d$  by coloring  $\mathcal{G}_d^n$  without conflict using  $k'$  colors, all node sets classified by the node color will be independent sets and the size of the maximum one will be larger than  $(n \log d)/d$ , a contradiction with Property 2.

The Corollary 3 reveals the lower bound of  $k$  by local methods for a random  $d$ -regular graph. Another important observation of  $k$  by (Achlioptas and Naor 2004) specifies that exact value of the chromatic number (i.e., the minimum  $k$ ) of a random  $d$ -regular graph. The property is described as follows:

**Property 3** ((Achlioptas and Naor 2004)). *Let  $t_d$  be the smallest integer  $t$  such that  $d < 2t \log t$ . The chromatic number of a random  $d$ -regular graph is either  $t_d$  or  $t_d + 1$ .*

It follows directly from Corollary 3 and Property 3 that, we can finish the proof of Corollary 1 by showing that the lower bound of  $k$  by local methods is always greater than the exact chromatic number:

$$d/\log d > t_d + 1 \text{ for } d \rightarrow \infty. \quad (2)$$

Let  $f(t) = 2t \log t$  and define  $t_0$  s.t.  $d = f(t_0) = 2t_0 \log t_0$ . Since  $t_d$  is the smallest integer  $t$  such that  $d < f(t)$ , we have  $f(t_0) = d \geq f(t_d - 1)$ . Since  $f$  is monotonically increasing,  $t_0 \geq t_d - 1$  and thus  $d/\log d - t_d - 1 \geq d/\log d - t_0 - 2$  always holds. Let  $d = 2t_0 \log t_0$ , we further derive the objective below:

$$\begin{aligned} d/\log d - t_d - 1 &\geq d/\log d - t_0 - 2 \\ &= \frac{2t_0 \log t_0}{\log(2t_0 \log t_0)} - t_0 - 2 > 0, \text{ for } d, t_0 \rightarrow \infty. \end{aligned}$$

we first prove that

$$\begin{aligned} \frac{\log t_0}{\log(2t_0 \log t_0)} &> 2/3 \\ \Rightarrow 3 \log t_0 &> 2 \log(2t_0 \log t_0) \\ \Rightarrow 3 \log t_0 &> 2(1 + \log t_0 + \log(\log t_0)) \\ \Rightarrow \log t_0 &> 2 + 2 \log(\log t_0) \text{ when } t_0 \rightarrow \infty. \end{aligned}$$

The above inequality holds obviously. Following the objective, we have:

$$\begin{aligned} \frac{2t_0 \log t_0}{\log(2t_0 \log t_0)} - t_0 - 2 \\ > \frac{4}{3}t_0 - t_0 - 2 > 0 \text{ when } t_0 \rightarrow \infty. \end{aligned}$$

Therefore, we finish the proof.  $\square$

### Proof of Corollary 2

We first recall the corollary.

**Corollary 2.**  *$L$ -AC-GNN is a  $L$ -local coloring method and thus a local coloring method*

*Proof.* Given an AC-GNN  $\mathcal{A}$  with  $L$  layers, let's consider a  $L$ -local equivalent node pair  $\{u, v\}$  in  $\mathcal{G}$  by an  $L$ -local automorphism  $\pi_L$ , which means that two rooted subtrees  $\mathcal{B}_{\mathcal{G}}(u, L)$  and  $\mathcal{B}_{\mathcal{G}}(v, L)$  are isomorphic and  $\mathbf{x}_w = \mathbf{x}_{\pi_L(w)}$  holds for every  $w \in \mathcal{B}_{\mathcal{G}}(u, L)$ . Since two rooted subtrees are isomorphic, the WL test (Weisfeiler and Lehman 1968) decides  $\mathcal{B}_{\mathcal{G}}(u, L)$  and  $\mathcal{B}_{\mathcal{G}}(v, L)$  are isomorphic and assigns the same color to  $w$  and  $\pi_L(w)$  for any  $w \in \mathcal{B}_{\mathcal{G}}(u, L)$ . To connect the WL test with AC-GNN, the following property is used:

**Property 4** ((Morris et al. 2019; Barceló et al. 2019; Xu et al. 2018a)). *If the WL test assigns the same color to two nodes in a graph, then every AC-GNN maps the two nodes into the same node embedding.*

Therefore,  $\mathcal{A}$  maps the  $u$  and  $v$  into the same node embedding. It follows that  $\mathcal{A}$  is  $L$ -local and thus local.  $\square$

### Proof of Property 3

We first recall the theorem.

**Property 3.** *Let  $\{u, v\}$  be a node pair in any graph  $\mathcal{G}$ , and  $L$  be any positive integer. If a  $L$ -AC-GNN discriminates  $\{u, v\}$ , a  $L^+$ -AC-GNN also discriminates it.*

Here, a  $L^+$ -AC-GNN is defined as an AC-GNN by stacking injective layers after  $L$ -AC-GNN (before  $CLS(\cdot)$ ). An injective layer includes a pair of injective aggregation function and injective combination function.

*Proof.* Let  $A^L$  be the  $L$ -AC-GNN that discriminates  $\{u, v\}$ , and  $\mathbf{h}_u^L, \mathbf{h}_v^L$  are the node embedding generated by  $A^L$  (before  $CLS(\cdot)$ ) and correspond to the node  $u, v$  respectively. Given the condition that  $A^L$  discriminates  $\{u, v\}$ , i.e.,  $\mathbf{h}_u^L \neq \mathbf{h}_v^L$ , we here consider the case where  $L^+$ -AC-GNN  $A^{L+}$  is an AC-GNN that only stack one injective layer after  $A^L$ .

Then,  $h_v^{L+}$ , the node embedding of  $v$  generated by  $A^{L+}$  is defined as:

$$h_v^{L+} = \text{COM}^{L+}(h_v^L, \text{AGG}^{L+}(\{h_m^L : m \in \mathcal{N}(v)\})), \quad (3)$$

where  $\text{COM}^{L+}$  and  $\text{AGG}^{L+}$  are the combination and aggregation functions of the newly stacked injective layer. Since  $h_u^L \neq h_v^L$ , and  $h_u^L, h_v^L$  are in the input multisets  $\{h_u^L, \text{AGG}^{L+}(\{h_m^L : m \in \mathcal{N}(u)\})\}, \{h_v^L, \text{AGG}^{L+}(\{h_m^L : m \in \mathcal{N}(v)\})\}$  respectively, the input multiset of  $\text{COM}^{L+}$  when calculating  $h_v^{L+}$  is different with the one when calculating  $h_u^{L+}$ . Because  $\text{COM}^{L+}$  is injective, we can further conclude that the output of  $\text{COM}^{L+}$  when calculating  $h_v^{L+}$  is different with the one when calculating  $h_u^{L+}$ , that is,  $h_u^{L+} \neq h_v^{L+}$ . By induction, the inequality can be applied for any additional stacked layers. We finish the proof.  $\square$

## Proof of Theorem 2

We first recall the theorem.

**Theorem 2.** *Let  $\mathcal{A}$  be a simple AC-GNN and both input and output of each layer in  $\mathcal{A}$  be the probability distribution  $\mathbf{h} \in \mathbb{R}^k$  of  $k$  colors,  $\mathcal{A}$  is color equivariant if and only if the following conditions hold:*

- *For any layer  $i$ , all the off-diagonal elements of  $\mathbf{C}^{(i)}$  are tied together and all the diagonal elements are equal as well. That is,*

$$\begin{aligned} \mathbf{C}^{(i)} &= \lambda_C^{(i)} \mathbf{I} + \gamma_C^{(i)} (\mathbf{I}\mathbf{I}^\top) \\ \lambda_C^{(i)}, \gamma_C^{(i)} &\in \mathbb{R} ; \mathbf{I} = [1, \dots, 1]^\top \in \mathbb{R}^k. \end{aligned} \quad (4)$$

- *For any layer  $i$ , all the off-diagonal elements of  $\mathbf{A}^{(i)}$  are also tied together and all the diagonal elements are equal as well. That is,*

$$\begin{aligned} \mathbf{A}^{(i)} &= \lambda_A^{(i)} \mathbf{I} + \gamma_A^{(i)} (\mathbf{I}\mathbf{I}^\top) \\ \lambda_A^{(i)}, \gamma_A^{(i)} &\in \mathbb{R} ; \mathbf{I} = [1, \dots, 1]^\top \in \mathbb{R}^k. \end{aligned} \quad (5)$$

- *For any layer  $i$ , all elements in  $\mathbf{b}^{(i)}$  are equal. That is,*

$$\mathbf{b}^{(i)} = \beta^{(i)} \mathbf{I} \quad \beta^{(i)} \in \mathbb{R} \quad \mathbf{I} = [1, \dots, 1]^\top \in \mathbb{R}^k. \quad (6)$$

*Proof.* Let  $\text{AGG}^{(i)}$  and  $\text{COM}^{(i)}$  be the aggregation and combination functions in the  $i_{th}$  layer of  $\mathcal{A}$ .  $\mathcal{A}$  is color equivariant if and only if all functions in  $\{\text{AGG}^{(i)}, \text{COM}^{(i)} : i \in 1, \dots, L\}$  are color equivariant. the aggregation function is color equivariant clearly and thus we are left to consider the color equivariance of combination functions. Considering the definition of color equivariant in Definition 4, the color equivariance of combination function  $\text{COM}^{(i)} = \sigma(\mathbf{x}\mathbf{C}^{(i)} + \mathbf{y}\mathbf{A}^{(i)} + \mathbf{b}^{(i)})$  is given by:

$$\sigma(\mathbf{x}\mathbf{C}^{(i)} + \mathbf{y}\mathbf{A}^{(i)} + \mathbf{b}^{(i)})\mathbf{P} = \sigma(\mathbf{x}\mathbf{P}\mathbf{C}^{(i)} + \mathbf{y}\mathbf{P}\mathbf{A}^{(i)} + \mathbf{b}^{(i)}). \quad (7)$$

$\text{COM}^{(i)}$  is color equivariant if and only if the equation above holds for any permutation matrix  $\mathbf{P} \in \mathbb{R}^{k \times k}$  and any vectors  $\mathbf{x}, \mathbf{y}$ . Considering it holds for any vectors  $\mathbf{x}, \mathbf{y}$ , We first find three special cases of  $\mathbf{x}$  and  $\mathbf{y}$ , which are necessary conditions and correspond to three conditions respectively:

*Case 0.* When  $\mathbf{y} = \vec{0}$ , we have that  $\sigma(\mathbf{x}\mathbf{C}^{(i)})\mathbf{P} = \sigma(\mathbf{x}\mathbf{P}\mathbf{C}^{(i)})$  holds for any  $\mathbf{P}$  and  $\mathbf{x}$ . That is,  $\mathbf{x}(\mathbf{C}^{(i)}\mathbf{P} - \mathbf{P}\mathbf{C}^{(i)}) = \vec{0}$  always holds, which reveals that  $\mathbf{C}^{(i)}\mathbf{P} = \mathbf{P}\mathbf{C}^{(i)}$ .  $\mathbf{C}^{(i)}\mathbf{P} = \mathbf{P}\mathbf{C}^{(i)}$  holds for any  $\mathbf{P}$  follows that  $C_{m,m}^{(i)} = C_{n,n}^{(i)}$  and  $C_{m,n}^{(i)} = C_{n,m}^{(i)}$  for any  $m, n \in \{1, \dots, k\}$ . Therefore, all the off-diagonal elements of  $\mathbf{C}^{(i)}$  are tied together and all the diagonal elements are equal as well.

*Case 1.* When  $\mathbf{x} = \vec{0}$ , we can prove that all the off-diagonal elements of  $\mathbf{A}^{(i)}$  are tied together and all the diagonal elements are equal as well following the similar induction in case 1.

*Case 2.* When  $\mathbf{x} = \mathbf{y} = \vec{0}$ , we have that  $\sigma(\mathbf{b}^{(i)})\mathbf{P} = \sigma(\mathbf{b}^{(i)})$  holds for any  $\mathbf{P}$ . Therefore, all elements in  $\mathbf{b}^{(i)}$  are equal.

After proving that these conditions are necessary for a color equivariant  $\mathcal{A}$ , we proceed to prove that the conditions above are already sufficient. Let  $\mathbf{C}^{(i)} = \lambda_C^{(i)} \mathbf{I} + \gamma_C^{(i)} (\mathbf{I}\mathbf{I}^\top)$ ,  $\mathbf{A}^{(i)} = \lambda_A^{(i)} \mathbf{I} + \gamma_A^{(i)} (\mathbf{I}\mathbf{I}^\top)$  and  $\mathbf{b}^{(i)} = \beta^{(i)} \mathbf{I}$ ,  $\text{COM}^{(i)}$  is then calculated by:

$$\begin{aligned} \text{COM}^{(i)}\mathbf{P} &= \sigma(\mathbf{x}\mathbf{C}^{(i)} + \mathbf{y}\mathbf{A}^{(i)} + \mathbf{b}^{(i)})\mathbf{P} \\ &= \sigma(\mathbf{x}\lambda_C^{(i)}\mathbf{I}\mathbf{P} + \mathbf{x}\gamma_C^{(i)}(\mathbf{I}\mathbf{I}^\top)\mathbf{P} + \mathbf{y}\lambda_A^{(i)}\mathbf{I}\mathbf{P} \\ &\quad + \mathbf{y}\gamma_A^{(i)}(\mathbf{I}\mathbf{I}^\top)\mathbf{P} + \beta^{(i)}\mathbf{I}\mathbf{P}) \\ &= \sigma(\mathbf{x}\mathbf{P}\lambda_C^{(i)}\mathbf{I} + \mathbf{x}\mathbf{P}\gamma_C^{(i)}(\mathbf{I}\mathbf{I}^\top) + \mathbf{y}\mathbf{P}\lambda_A^{(i)}\mathbf{I} \\ &\quad + \mathbf{y}\mathbf{P}\gamma_A^{(i)}(\mathbf{I}\mathbf{I}^\top) + \beta^{(i)}\mathbf{I}) \\ &= \sigma(\mathbf{x}\mathbf{P}\mathbf{C}^{(i)} + \mathbf{y}\mathbf{P}\mathbf{A}^{(i)} + \mathbf{b}^{(i)}). \end{aligned} \quad (8)$$

Therefore,  $\text{COM}^{(i)}$  is color equivariant if and only if the conditions hold, which completes the proof.  $\square$

## Related Works

### Graph Neural Networks.

**Analysis on the power of GNNs.** With the overwhelming success of GNNs in various fields ranging from recommendation system and VLSI design, recently, the study on the power of GNNs becomes more and more important and necessary, and has attracted extensive interest. The two recent papers (Morris et al. 2019; Xu et al. 2018a) formalize the power as the capability to map two equivalent nodes to the same node embedding. They explore the power by establishing a close connection between GNNs and 1-Weisfeiler-Lehman (WL) test, a classical algorithm for the graph isomorphism test. More specifically, they independently showed that every time when two nodes are assigned the same embedding by any GNN, the two nodes will always be labeled the same by the 1-WL test, which means that GNNs are upper-bounded by 1-WL test in terms of the representation power. To develop a more powerful GNN that breaks through the limit by 1-WL test, many attempts are made from different perspectives. Some GNNs (Chen et al. 2019; Maron et al. 2019, 2018; Morris et al. 2019) are proposed by mimicking a higher-order-WL test based on higher-order tensors. Another direction is to introduce more

informative features/operations to make the model sensitive to the substructure (Li et al. 2020a) or global structure (Barceló et al. 2019; You, Ying, and Leskovec 2019; You et al. 2021). We leave the detailed discussion of such a non-local scheme in Appendix . Besides the study on the comparison with WL-test, many other works investigate the power of GNNs from different angles and a lot of interesting conclusions are obtained. Xu et al. (Xu et al. 2019) shows that GNNs align with DP and thus are expected to solve tasks that are solvable by DP. This interesting conclusion leaves us a future work to study GNN in the coloring problem by learning previous DP-based coloring algorithms. Loukas et al. (Loukas 2019) concludes that the product of the GNN’s depth and width must exceed a polynomial of the graph size to obtain the optimal solution of some problems, e.g., Maximum Independent Set (MIS) problem, and coloring problem. This conclusion motivates our experiments on the model depth, which is covered in Appendix . Another work (You, Ying, and Leskovec 2020) explores the design space for GNNs and gives some best parameters in various design dimensions, where best means the selected parameters make the corresponding GNNs more effective than others. We follow the guidance of this work to select most hyper-parameters and model architectures, as shown in Appendix . GeomGCN (Pei et al. 2020) points the limits of AC-GNNs from the perspective of network geometry, the node can only exchange information with its neighbors, while the long-range dependencies are missed and similar nodes (may be very distant) are more likely to be proximal. To overcome the issues, a novel geometric aggregation scheme was proposed. Generally, instead of aggregating information from graph neighborhoods directly, the original graph is mapped to a latent continuous space according to pre-calculated node embedding. Then, a structural neighbor relation is constructed based on the distance and relative direction in the latent space. However, their motivation is not applicable for the coloring problem: the coloring results are totally not relevant with the similarity of nodes.

**GNNs for NP problem.** Recently, the applications of GNNs on NP problems received great attention. Some works integrate GNNs to a sophisticated heuristic algorithm designed for a specific NP problem. Li et al. (Li, Chen, and Koltun 2018) proposes a GNN-based framework to solve the MIS problem, where the adopted GNN generates multiple probability maps to represent the likelihood of each vertex being in the optimal solution. However, the following heuristic algorithm to handle the *multiple* probability maps is time-consuming. In their experiments, a graph with 1,000 vertices will yield up to 100K diverse solutions and the heuristic algorithm is processed up to 10 minutes. Not saying that the runtime may explode when applied in the  $k$ -coloring problem. Another work (Lou et al. 2020) uses GNNs to solve the subgraph matching problem, a problem of determining whether a given query graph is a subgraph of a large target graph. They designed a particular loss function, to ensure that the subgraph relations are preserved in the embedding space. Besides these direct applications, some theoretical works discussed the power of GNNs to solve the

NP problem. If  $P \neq NP$ , GNNs cannot exactly solve these problems. Under this assumption, Sato (Sato, Yamada, and Kashima 2019) demonstrates the approximation ratios of GNNs for some combinatorial problems such as the minimum vertex cover problem. They study the ratio by building the connection between GNNs and distributed local algorithms. Specifically, they show that the set of graph problems that GNN classes can solve is the same as the one that distributed local algorithm classes can solve. Besides a pure GNN, Dai et al. (Dai et al. 2017) develops a framework that combines reinforcement learning and graph embedding to address some NP problems. Generally, the reinforcement learning model uses the graph embedding obtained by Structure2Vec (Dai, Dai, and Song 2016).

**GNNs on tasks under heterophily.** To the best of our knowledge, Zhu et al. (Zhu et al. 2020b) is the first work that formally addressed the drawbacks of previous GNNs on tasks under heterophily. Beyond homophily, they proposed three designs that can be beneficial for the learning under heterophily: 1) The node embedding and aggregated embeddings should be separated. This statement aligns with our Property 2, addressing the limitation of an integrated AC-GNN in the coloring problem. Although most previous works focus on the homophily scenario, some of them (You, Ying, and Leskovec 2020; Hamilton, Ying, and Leskovec 2017) also pay attention to the separation of neighbor embeddings and ego-embedding (i.e., a node’s embedding). 2) The aggregation function should involve higher-order neighborhoods. The intuition is that higher-order neighborhoods may be homophily-dominant. Take the coloring problem as an example, if two nodes, say  $u, v$ , are connected with another same node  $t$ , then  $u, v$  are more likely to be assigned the same color. This design is also employed in previous works (Abu-El-Haija et al. 2019; Defferrard, Bresson, and Vandergheynst 2016) for homophily, considering that a higher order polynomials of the normalized adjacency matrix indicates a low-pass filter. 3) The final results should combine intermediate representations from all layers. The design is originally introduced in jumping knowledge networks (Xu et al. 2018b) and motivated by the fact that each layers contains information from neighborhoods of different depth. Zhu also proposes another method for tasks under heterophily (Zhu et al. 2020a). In this work, they also gives a prior that the feature represents the probability(belief). The method is based on the belief propagation based on the trainable compatibility matrix. Interestingly, if we dismiss the color equivariance in the summarized rules and still keeps the prior of the belief, we can directly build the same model with the one used in (Zhu et al. 2020a).

## Coloring methods.

The graph coloring problem is crucial in domains ranging from network science and database systems to VLSI design. Here, we classify previous coloring methods as learning-based methods and non-learning-based methods.

**Non-learning-based methods.** As a classical problem in the NP-hard classes and graph theory, graph coloring problem has received considerable attention in past decades.

Here, we only cover some representative non-learning-based methods that are related to our method from some perspectives. Braunstein et al. (Braunstein et al. 2006) proposed Belief propagation (BP) and Survey propagation (SP) to solve the  $k$ -coloring problem, where both methods belong to a message-passing scheme. The key idea is that, each node is randomly assigned a probability distribution of colors, then the probability is updated based on the probabilities of neighbors. Formally, define  $\eta_{e \rightarrow u}^k$  as the probability that edge  $e = \{u, v\}$  refutes  $u$  as the color  $k$ , for the  $k$ -coloring problem,  $\eta_{e \rightarrow u}^k$  is updated by:

$$\eta_{e \rightarrow u}^k = \frac{\prod_{v' \in \mathcal{N}(v)/u} (1 - \eta_{\{v, v'\} \rightarrow v}^k)}{\sum_{r=1}^k \prod_{v' \in \mathcal{N}(v)/u} (1 - \eta_{\{v, v'\} \rightarrow v}^r)} \quad (9)$$

The numerator indicates the possibility that  $v$  is colored by the color  $k$  (without considering node  $u$ ). And the fraction is for normalization, making that the sum equals to one. The SP procedure is a little different, it did not normalize the probability directly, but introduced a joker state,  $\eta_{e \rightarrow u}^*$ , representing that the edge can not refute any colors, i.e.,  $1 = \eta_{e \rightarrow u}^* + \sum_{r=1}^k \eta_{e \rightarrow u}^r$ . The method is simple and very close to our non-training version. However, the method is more theoretical and less practical because it is easy to fall into a trivial solution, i.e., all edges are assigned into the joker state. Even though a non-trivial solution can be found, a large number of iterations may be required due to its randomness. Apart from message passing, Takefuji (Takefuji and Lee 1991) proposed an Artificial Neural Network (ANN) based method for the four-coloring problem. The basic conclusion is that the probability distribution<sup>1</sup> can be updated by subtracting the aggregated probability distributions of neighbors, which aligned with the intuition for our parameter initialization.

**Learning-based methods.** Although our work is the first one that tries and analyzes the power of GNNs in the graph coloring problem, there is a surge of learning-based methods for coloring. Lemos et al. (Lemos et al. 2019) integrated Recurrent Neural Networks (RNNs) into the message passing framework, i.e., two RNNs were employed to compute the embedding update from aggregated messages for each vertex and color. Finally, the graph embedding was used to predict the chromatic number, and the node embedding was used to predict exact node color by clustering. However, the clustering-based method generated a prohibitive conflict number as shown in Table 1 of our paper, making the method not practical. Huang et al. (Huang, Patwary, and Diamos 2019) introduced a fast heuristics coloring algorithm using deep reinforcement learning. For each step (state), the model predicts the next node and its best color solution with a win/lose feedback. The prediction depends on previous coloring results and a graph embedding generated by an LSTM. The method can give relatively accurate coloring results, but still only comparable with some simple heuristic algorithms such as dynamic order coloring. On the contrary,

<sup>1</sup>In their work, the node attribute is not probability distribution but a binary vector indicating the selected colors. Nevertheless, the conclusion still holds for a probability case.

---

#### Algorithm 1: ITERATIVEREMOVAL

---

**Require:**  $\mathcal{G} = \{\mathcal{V}, \mathcal{E}\} \rightarrow$  Target graph.

**Require:**  $k \rightarrow$  Number of available colors.

- 1: **while**  $\exists u \in \mathcal{V}$  s.t. degree of  $u < k$  **do**
  - 2:     Update degree of the neighbor of  $u$  by subtracting one.
  - 3:     Remove  $u$  in  $\mathcal{G}$ .
  - 4: **end while**
- 

our supplementary results in Appendix demonstrates that our method outperforms these simple heuristic algorithms significantly. Zhou et al. (Zhou, Hao, and Duval 2016) also borrowed the idea of reinforcement learning. However, the proposed method did not use a training scheme: the actions towards the environment is defined by a deterministic update function of the coloring probability distributions. The method achieves a state-of-the-art result quality. However, the framework contains a descent-based local search with a portion of randomness, which requires a repeated execution with different random seeds. Moreover, the local search algorithm may require extensive iterations to find a local optimum. Due to these limitations, the method suffers from the runtime, in their experiments, the coloring process for a 500-node graph costs more than 100 seconds.

## Preprocess & Postprocess

In our method, we add preprocess and postprocess procedures to reduce the problem complexity and improve the result quality. Note that these techniques are not necessary for our method, in Appendix , we list the experimental results without any postprocess procedures. At the same time, we have implemented these techniques in DGL or by a series of tensor operations, so that both of them can be efficiently processed by GPU.

**Preprocess** In the preprocess part, we remove the node with a degree less than  $k$  iteratively. Because a node with degree less than  $k$  will always not contribute to a conflict in the optimal solution, this kind of removal will not introduce any redundant conflicts. The algorithm is shown in Algorithm 1. There are many other graph simplification techniques in the practical applications such as bridge detection (Li et al. 2019), we do not focus on these techniques, because the aim of our work is not to develop a very effective coloring method by powerful pre-process and post-process procedures, but to study the power of GNNs on the coloring problems.

**Postprocess** In the postprocess part, we iteratively detect 1) whether a color change in a single node will decrease the conflict number or 2) whether a swap of colors between connected nodes will decrease the conflict number. The algorithm is shown in Algorithm 2. Generally, we iteratively check (L2 - L18) each node (L4 - L11) and each conflict edge (L12 - L17), if one better solution is found, we modify the coloring result to the better one and continue the iteration.

---

**Algorithm 2: POSTPROCESS**


---

**Require:**  $\mathcal{G} = \{\mathcal{V}, \mathcal{E}\} \rightarrow$  Target graph.

**Require:**  $f \rightarrow$  Coloring results.

```

1: Is_changed  $\leftarrow$  True;
2: while Is_changed do
3:   Is_changed  $\leftarrow$  False;
4:   for  $u \in \mathcal{V}$  do
5:     for  $r \in \{1, \dots, k\}$  do
6:       if the conflict # reduces when set  $f(u)$  to  $r$  then
7:          $f(u) \leftarrow r$ ;
8:         Is_changed  $\leftarrow$  True;
9:       end if
10:    end for
11:  end for
12:  for  $e = \{u, v\} \in \mathcal{E}$  do
13:    if the conflict # reduces when swap color of  $u, v$  then
14:      swap color of  $u, v$ ;
15:      Is_changed  $\leftarrow$  True;
16:    end if
17:  end for
18: end while

```

---

### Global method

During the exploration of GNNs, the locality of GNNs has been widely observed as an intrinsic nature. The main concern in previous works is that the locality inhibits GNNs from detecting the global graph structure, thereby harming the representation power. In the paper, we discuss one representative "global" technique: deep layers, and show that it can enhance the discrimination power while still cannot make AC-GNNd always global. In this section, we use the notation of the local method defined in our paper, and look back on previous solutions to see whether they provide a truly global scheme by our definition. We hope that our analysis can provide some insights on the global GNNs for future research. We first recap the definition of a local method:

**Definition 3** (local method (Gamarnik and Sudan 2014)). *A coloring method  $f$  is  $r$ -local if it fails to discriminate any  $r$ -local equivalent node pair. A coloring method  $f$  is local if  $f$  is  $r$ -local for at least one positive integer  $r$ .*

To determine whether a coloring method is local or not, we need to, by definition, determine whether the method is able to discriminate two local equivalent nodes. Consider a local equivalent node pair, say  $u, v$ , we can exam previous global methods by testing whether the node embeddings of  $u$  and  $v$  are the same. To simplify the discussion and only focus on the main point, we summarize and distill the most representative techniques as follows:

#### Distance encoding (Li et al. 2020a).

Distance Encoding is a general class of structure-related features to enrich the sub-structure or even global structure information. In their work, the distance can be represented in various forms and the distance encoding can be used in two different ways, i.e., extra node features and a controller for message passing. For simplicity, we only consider the case where shortest path distance is used to measure distance and

employed as the extra node features. Formally, the input features with distance encoding is:

$$\mathbf{h}_v^0 = \mathbf{x}_v^0 \oplus \sum_{v \in \mathcal{S}} d(u, v) \quad (10)$$

Here,  $\mathbf{x}_v^0$  is the original node attribute,  $d(u, v)$  is the shortest path distance between  $u$  and  $v$ ,  $\oplus$  is the concatenation mark, and  $\mathcal{S}$  is the target structure defined in the original paper, which can be the whole graph, i.e.,  $\mathcal{S} = \mathcal{V}$ , or a substructure, i.e.,  $\mathcal{S} \in \mathcal{V}$ . We make the following statements:

**Property 4.** *AC-GNNs enhanced by distance encoding ARE global.*

*Proof.* Note that a local method cannot discriminate *any* local equivalent node pair. We can finish the proof by contradiction. Assume there exists  $r > 0$  such that the enhanced AC-GNN is a  $r$ -local method, i.e., it fails to discriminate any  $r$ -local equivalent node pair. We build a connected graph containing  $2r + 3$  nodes like a linked list. A figure illustration is given in Figure 1, where the number represents the node index. Assume all nodes share the same node attribute, i.e.,  $\mathbf{x}_i^0 = \mathbf{x}_j^0, \forall i, j \in \{0, \dots, 2r + 2\}$ . Consider the two nodes,  $v_r$  and  $v_{r+1}$ , their depth- $r$  neighborhood are topologically equivalent, i.e.,  $\mathcal{B}_G(v_r, r) = \mathcal{B}_G(v_{r+1}, r)$ . Therefore,  $\{v_r, v_{r+1}\}$  is a  $r$ -local equivalent node pair. However, the distance encoding of the two nodes are different, where  $\sum_{v \in \mathcal{G}} d(v_r, v) = r^2 + 3r + 3$  but  $\sum_{v \in \mathcal{G}} d(v_{r+1}, v) = r^2 + 3r + 2$ , resulting in a difference between  $\mathbf{h}_r^0$  and  $\mathbf{h}_{r+1}^0$ . Similarly, the neighbors of  $v_r$  and  $v_{r+1}$  have the different distance encodings. Therefore, the distance encoding makes the two local equivalent nodes differentiable by providing a different input for both aggregation and combination functions, which completes the proof.  $\square$

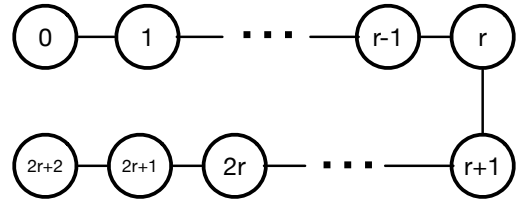

Figure 1: A contradiction example to prove that the distance encoding makes an AC-GNN global.

#### Readout function (Barceló et al. 2019).

Barcel et al. (Barceló et al. 2019) proposed a scheme to update node features by aggregating not only neighbor information, but also the global attribute vector. The function considering a global attribute vector is also called the readout function. In their work, it is demonstrated that even a very simple readout function, i.e., summation of all node features, can capture all FOC<sub>2</sub> classifiers, which means that the representation power is improved. Indeed, the global

<sup>2</sup>We do not discuss extreme cases here, e.g.  $\text{COM}(\cdot) = 0$ .

feature vectors contain some information across the whole graph, and the distance encoding discussed in Section is also a kind of readout function in the form of distance measurement. But can we declare that *AC-GNNs become global methods as long as we use a readout function*? Here, we discuss the simplest form used in (Barceló et al. 2019), aggregate-combine-readout GNNs (ACR-GNNs), where the readout is calculated by the summation of all node features. An ACR-GNN is formalized as follows:

$$\begin{aligned} \mathbf{h}_v^{(i)} = & \text{COM}^{(i)}(\mathbf{h}_v^{(i-1)}, \text{AGG}^{(i)}(\{\mathbf{h}_u^{(i-1)} : u \in \mathcal{N}(v)\}), \\ & \text{READ}^{(i)}(\{\mathbf{h}_u^{(i-1)} : u \in \mathcal{V}\})), \end{aligned} \quad (11)$$

We make the following statement:

**Property 5.** *ACR-GNNs are NOT global.*

*Proof.* The intuition for proof comes from the fact that the used readout function, i.e., summation of all node features, keeps the same for all nodes. We first prove the following:

**Corollary 4.** *If an ACR-GNN succeeds in discriminating a node pair, an AC-GNN will also discriminate it.*

Given a node pair  $\{u, v\}$  in the graph  $\mathcal{G}$ . Let  $\mathbf{h}_u^{(k)'} and  $\mathbf{h}_u^{(k)}$  represents the node embedding of  $u$  after  $k$  layers by an ACR-GNN  $\mathcal{A}'$  and an AC-GNN  $\mathcal{A}$  respectively. Suppose after  $k$  layers,  $\mathcal{A}'$  discriminate them, i.e.,  $\mathbf{h}_u^{(k)'} \neq \mathbf{h}_v^{(k)'}$ , while  $\mathcal{A}$  fails to discriminate them, i.e.,  $\mathbf{h}_u^{(k)} = \mathbf{h}_v^{(k)}$ . It follows that during the layer  $t$  from 0 to  $k-1$ ,  $\mathbf{h}_u^{(t)'} = \mathbf{h}_v^{(t)'}$  and  $\mathbf{h}_u^{(t)} = \mathbf{h}_v^{(t)}$ . That is, for any  $t$  from 0 to  $k-1$ , we can create a valid mapping  $\phi$  such that  $\mathbf{h}_v^{(t)'} = \phi(\mathbf{h}_v^{(t)})$  for any node  $v \in \mathcal{V}$ .$

Consider the inequality after  $k$  layers, since node  $u$  and  $v$  always have the same readout term, i.e.,  $\text{READ}^{(k)}(\{\mathbf{h}_u^{(k-1)'} : u \in \mathcal{V}\})$ , combining with Equation 11, it must be the case that:

$$\begin{aligned} (\mathbf{h}_v^{(k-1)'}, \{\mathbf{h}_s^{(k-1)'} : s \in \mathcal{N}(v)\}) & \neq \\ (\mathbf{h}_u^{(k-1)'}, \{\mathbf{h}_s^{(k-1)'} : s \in \mathcal{N}(u)\}) \end{aligned} \quad (12)$$

That is,

$$\begin{aligned} (\phi(\mathbf{h}_v^{(k-1)}), \{\phi(\mathbf{h}_s^{(k-1)}) : s \in \mathcal{N}(v)\}) & \neq \\ (\phi(\mathbf{h}_u^{(k-1)}), \{\phi(\mathbf{h}_s^{(k-1)}) : s \in \mathcal{N}(u)\}) \end{aligned} \quad (13)$$

However, according to the assumption, the AC-GNN fails to discriminate the two nodes, indicating that the inequality above cannot hold. Hence we have reached a contradiction.

Therefore, we can conclude that the ACR-GNN also cannot discriminate any local equivalent node pair, making it a local method. Actually, this proof also demonstrates that such an ACR-GNN is upper-bounded by AC-GNNs in the terms of the discrimination power.  $\square$

## Identity-aware Graph Neural Networks (You et al. 2021).

Identity-aware Graph Neural Networks (ID-GNNs) focus on solving the problem that the embeddings are only related to

the local subtree. The key insight is to inductively consider the root node during message passing, i.e., whether the aggregated node is the target node itself. If the aggregated node is the target node, a different aggregation and combination channel is used so that the ID-GNN is a heterogeneous one. Formally, let the target node is  $u$ , i.e., we are calculating the node embedding of  $u$ , then, the mediate features of other nodes are given by:

$$\mathbf{h}_{v,u}^{(i)} = \text{COM}^{(i)}(\mathbf{h}_{v,u}^{(i-1)}, \{\text{AGG}_{\mathbf{1}[s=u]}^{(i)}(\mathbf{h}_{s,u}^{(i-1)}) : s \in \mathcal{N}(v)\}), \quad (14)$$

Here,  $\mathbf{h}_{v,u}^{(i)}$  represents the mediate feature of node  $v$  after  $i_{th}$  layer when calculating the node embedding of  $u$ ,  $\text{AGG}^{(i)}$  contains two functions, where  $\text{AGG}_1^{(i)}$  is applied to the target node, and  $\text{AGG}_0^{(i)}$  is for other nodes. The simple heterogeneous scheme makes the target node different from other nodes and therefore sensitive to the identity. However, such a scheme still fails to discriminate  $c, d$  in the Figure 1(a) of our paper. Based on this observation, we claim the following property:

**Property 6.** *ID-GNNs are NOT global.*

*Proof.* We can finish the proof by showing that ID-GNNs cannot discriminate any local equivalent node pair. Given an ID-GNNs  $\mathcal{A}$  with  $L$  layers, let's consider a  $L$ -local equivalent node pair  $\{u, v\}$  in  $\mathcal{G}$  by an  $L$ -local isomorphism  $\pi_L$ , which means that the two subgraphs  $\mathcal{B}_{\mathcal{G}}(u, L)$  and  $\mathcal{B}_{\mathcal{G}}(v, L)$  are isomorphic and  $\mathbf{x}_w = \mathbf{x}_{\pi_r(w)}$  holds for every  $w \in \mathcal{B}_{\mathcal{G}}(u, r)$ . Here, we propose a stronger property:

**Corollary 5.** *Given a  $L$ -depth ID-GNN and a  $L$ -local equivalent node pair  $\{u, v\}$  by  $\pi$ ,  $\mathbf{h}_{s,v}^i = \mathbf{h}_{\pi(s),u}^i$  holds for any iteration  $i$  and any node  $w \in \mathcal{B}_{\mathcal{G}}(u, r)$  if  $i + d(s, v) \leq L$ , where  $d$  represents the shortest distance.*

We prove the corollary by a nested induction.

**First induction:**

This statement, i.e.,  $\mathbf{h}_{s,v}^i = \mathbf{h}_{\pi(s),u}^i$ , apparently holds when  $i + d(s, v) \leq 0$ . Suppose this holds if  $i + d(s, v) \leq k$  (first assumption), we now prove that the statement will also hold when  $i + d(s, v) = k + 1$  as long as  $k + 1 \leq L$ .

**Induction in the induction:** For those nodes, say  $s_{k+1}$ , whose shortest distance with  $v$  is  $k + 1$ , i.e.,  $d(s_{k+1}, v) = k + 1$ , we have  $\mathbf{h}_{s_{k+1},v}^0 = \mathbf{h}_{\pi(s_{k+1}),u}^0$  since  $\{u, v\}$  is a  $L$ -local equivalent node pair and  $k + 1 \leq L$ . Suppose  $\mathbf{h}_{s,v}^i = \mathbf{h}_{\pi(s),\pi(v)}^i$  holds if  $i = t$  and  $d(s, v) = k + 1 - t$  (second assumption), we continue to prove that this will hold if  $i = t + 1$  and  $d(s, v) = k - t$ .

Consider those nodes, say  $s_{k-t}$ , whose shortest distance between  $v$  is  $k - t$ , i.e.,  $d(s_{k-t}, v) = k - t$ , then  $\mathbf{h}_{s_{k-t},v}^{t+1}$  is given by:

$$\begin{aligned} \mathbf{h}_{s_{k-t},v}^{t+1} = & \text{COM}^{(t+1)}(\mathbf{h}_{s_{k-t},v}^t, \\ & \{\text{AGG}_{\mathbf{1}[s=v]}^{(t+1)}(\mathbf{h}_{s,v}^t) : s \in \mathcal{N}(s_{k-t})\}), \end{aligned} \quad (15)$$

According to the first assumption,  $\mathbf{h}_{s_{k-t},v}^t = \mathbf{h}_{\pi(s_{k-t}),u}^t$  since  $i + d(s_{k-t}, v) = k$ . We then consider the second

term in Equation 15,  $\mathbf{h}_{s,u}^{(t)} : s \in \mathcal{N}(s_{k-t})$ . The distance between the neighbors of  $s_{k-t}$  and the root node  $v$  ranges from  $k - t - 1$  to  $k - t + 1$ . For the neighbor nodes  $s_{k-t-1} \in \mathcal{N}(s_{k-t})$  with a distance  $k - t - 1$  between  $v$ , we have  $\mathbf{h}_{s_{k-t-1},v}^t = \mathbf{h}_{\pi(s_{k-t-1}),u}^t$  since  $t + d(s_{k-t-1}, v) = k - 1 \leq k$  (first assumption). Similarly, for the neighbor nodes  $s'_{k-t} \in \mathcal{N}(s_{k-t})$ , the equation still holds since  $t + d(s'_{k-t}, v) = k \leq k$  (first assumption). For the neighbor nodes  $s_{k-t+1} \in \mathcal{N}(s_{k-t})$ , the equation  $\mathbf{h}_{s_{k-t+1},v}^t = \mathbf{h}_{\pi(s_{k-t+1}),u}^t$  also holds since  $i = t$  and  $d(s_{k-t+1}, v) = k + 1 - t$  (second assumption).

**End of the induction in the induction:** Hence by mathematical induction  $\mathbf{h}_{s,v}^i = \mathbf{h}_{\pi(s),\pi(v)}^i$  is correct for all positive integers  $i$  and  $d(s, v)$ . Therefore, we show that  $\mathbf{h}_{s,v}^i = \mathbf{h}_{\pi(s),\pi(v)}^i$  holds when  $i + d(s, v) = k + 1 \leq L$ ,  $d(s, v)$  and  $i$  are positive integers.

**End of the induction:** Hence by mathematical induction,  $\mathbf{h}_{s,v}^i = \mathbf{h}_{\pi(s),u}^i$  holds for any iteration  $i$  and any node  $w \in \mathcal{B}_G(u, r)$  if  $i + d(s, v) \leq L$ , such completes the proof of Corollary 5.

Based on Corollary 5, we can conclude that  $\mathbf{h}_{v,v}^L = \mathbf{h}_{u,u}^L$ , indicating that the  $L$ -depth ID-GNN fails to discriminate  $u$  and  $v$ , which completes the proof.  $\square$

## Randomness.

In the development of GNNs, random schemes are widely-used and studied. Ryoma et al. (Sato, Yamada, and Kashima 2020) and Andreas et al. (Loukas 2019) both prove that the distinct node attributes (even initialized randomly) enhance the representation power significantly. George et al. (Dasoulas et al. 2019) propose a randomly coloring methods to distinguish different nodes and break the local equivalence. Position-aware GNN (You, Ying, and Leskovec 2019) makes use of the distance encoding to design a position-aware GNN, where one of the differences between distance encoding (Li et al. 2020a) is that the distance is not measured with a pre-defined set  $\mathcal{S}$ , but with a set of *randomly* selected anchor node sets. In our work, we also demonstrated that the randomness enhances the discrimination power of AC-GNNs, because nodes are not possible to be local equivalent considering that their node attributes are initialized randomly. Therefore, we want to know:

**Q:** Does randomness make AC-GNNs global?

Unfortunately, we are not able to answer the question now. We can only declare that a random scheme indeed helps to distinguish local equivalent node pair, but it *may* be still local. The reason is that the AC-GNNs are not deterministic anymore if we add some randomness, therefore, the definition of local methods is not available here. In some cases, the upper bound (or lower bound) remains when the function becomes not deterministic, but a formal proof is needed in our case. We look forward to a deeper discussion on the discrimination power of randomness in AC-GNNs, and leave this as our future work.

## Supplementary Experiments

### Experiment & model settings.

**Experiments.** We implemented our experiments in the PyTorch Deep Graph Library (DGL) (Wang et al. 2019). We conducted all experiments on a server with a Titan X GPU and an E5-2630 2.6 GHz CPU. Besides GNN-GCP and tabucol compared in the paper, we also implement integer linear programming (ILP) based solver by Gurobi (OPTIMIZATION 2014), and three heuristics coloring methods which are used as baselines in (Huang, Patwary, and Damos 2019). In the supplementary experiments, 80% randomly selected samples in the layout dataset are separated into the training dataset (for trainable models) and the testing dataset contains the remaining samples. In the paper, we only run our model once with a specified  $k$  and obtain the cost (conflict number), in the supplementary experiments, we sometimes need to calculate the chromatic number by our model, i.e., calculate the minimum  $k$  that achieves a zero cost. To do this, we iteratively run our model and add  $k$  by one after each iteration until a zero cost is received.

**Network and training.** A detailed network and training setting is covered in the Appendix. Layout dataset is used as the training data and we will show that our GDN trained on these small graphs can generalize to much larger ones such as Citation dataset. Other datasets are comprised of either (1) a single graph, or (2) graphs with varying chromatic numbers, which are not suitable for training, especially for other variations. During training, we initialize the variables of GDN in each layer as:

$$\lambda_C^{(i)} = 1, \gamma_C^{(i)} = 0, \lambda_A^{(i)} = -1, \gamma_A^{(i)} = 0, \beta^{(i)} = 0 \quad (16)$$

The initialization is motivated by the truth that neighbors of each node should be assigned as different colors as the node.

**Model hyperparameters.** If not specified, all AC-GNN variations have 2 layers and the hidden dimension is 64. Other training parameters of these variations keep the same with our proposed GDN. We use the Adam (Kingma and Ba 2014) optimizer with a 1024 batched graph (if batch-graph is possible) and a learning rate 0.001. Training proceeds for 10 epochs and takes about one hour. More detailed default hyperparameter values can be found in our released code, i.e., `color_arg.py`.

**Datasets.** We totally evaluate performance on five datasets.

(1) The layout dataset, which is composed of many simplified small but dense layout graphs transformed from circuit layout. This dataset is widely used as the benchmark for the layout decomposition problem (Jiang and Chang 2017; Li et al. 2020b; Yu et al. 2015), a similar problem in the industry manufacturing based on the graph coloring problem. The number of available colors  $k$  is set to 3 following previous works;

(2) The citation networks (Cora, Citeseer, and Pubmed) (Sen et al. 2008) that contains real-world graphs from academic search engines. We follow the setting in (Li, Chen, and Koltun 2018) and regard them as the coloring scenario



for large but sparse graphs, hence dismissing their original node attributes and edge directions.  $k$  in Cora, Citeseer, and Pubmed are set to 5, 6 and 8 respectively;

(3) Three random graph distributions namely: random power-law tree, Watts-Strogatz small-world and Holme and Kim model (Watts and Strogatz 1998; Holme and Kim 2002), some works (Lemos et al. 2019) evaluated them on the graph coloring problem.  $k$  is set from 2 to 5 due to its randomness. The settings to generate the random graphs are: random power-law tree ( $\gamma=3$ ), Watts- Strogatz small-world ( $k = 4$ ,  $p = 0.25$ ) and Holme and Kim model ( $m = 4$ ,  $p = 0.1$ ). To fit the problem context and prevent miscalculations, we removed all self-loops in the testing graphs and added duplex connections between connected nodes;

(4) COLOR dataset<sup>3</sup> that contains medium sized graphs, which is also the most essential dataset in the graph coloring community (Lemos et al. 2019; Gualandi and Malucelli 2012; Wu and Hao 2012). Here, we select instances following (Lemos et al. 2019), other instances show a similar trend in our experiments;

(5) Regular dataset that contains  $d$ -regular graphs with size  $n$ . We use NetworkX (Hagberg, Schult, and Swart 2008) to randomly generate 100 graphs whose density is 16 and graph size is 128. The color number is set to  $d/\log d + 1 = 5$ .

For some tasks (Random, Citation) whose available color numbers  $k$  are not specified, we assign  $k$  as the chromatic numbers of graphs, which are obtained from the CSP Solver<sup>4</sup>. Each graph  $G$  is first preprocessed by removing vertices iteratively following steps in (Yu et al. 2015; Jiang and Chang 2017).

### Comparison with other methods.

We compare our method with the other three heuristics coloring methods use in (Huang, Patwary, and Damos 2019) and ILP based method. We only compare these methods in the layout dataset, because ILP even cannot solve others within 24 hours. The three heuristic algorithms are summarized as follows:

**Static-ordered:** Coloring nodes in the order of node IDs.

**Sorted-ordered:** Coloring nodes in the largest degree first manner.

**Dynamic-ordered:** Coloring nodes in the largest degree first manner, while the degree is updated when coloring nodes, i.e., the neighbors of the colored node will decrease their degree by one.

The results are shown in Figure 2. We measure the average predicted  $k$  (minimal color number to be conflict-free) on four different graph size  $|\mathcal{V}|$ , i.e., small ( $|\mathcal{V}| < 8$ ), Medium ( $8 \leq |\mathcal{V}| < 16$ ), Large ( $16 \leq |\mathcal{V}| < 32$ ), Huge ( $32 \leq |\mathcal{V}|$ ). All methods contain a pre-process procedure for a fair comparison. From the results, we can see that *Our method achieves exactly the same performance with ILP in all graphs except the huge one*. Note that ILP is an optimal coloring solver, indicating that our method reaches the optimality for relatively small graphs. However, even for such small cases, three heuristic algorithms fail to be close to ILP

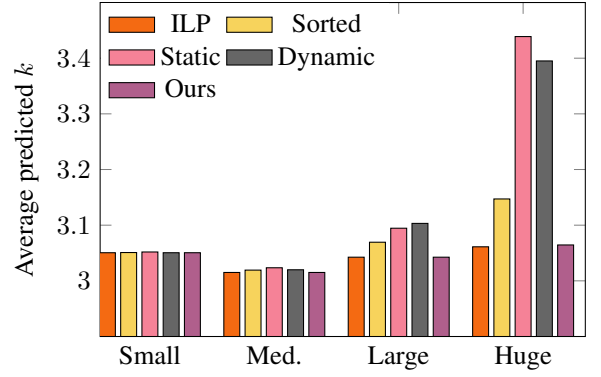

Figure 2: Comparison with other heuristic methods.

or our method. For large and huge graphs, the average  $k$  is increased by more than 10% for static and dynamic algorithms. With the growth of the graph size, our method becomes more and more advanced compared with these heuristic algorithms.

### Ablation study

**Model depth** In our paper, we show that a deep AC-GNN is a more powerful coloring solver (Property 3). Here, we validate our conclusion by experiments. The results on layout dataset are shown in Figure 3, where the solved ratio is defined as in paper, i.e., the ratio between the number of edges without introducing conflicts and the number of total edges. According to the results, we can conclude that a deeper model indeed has a more positive influence on the results. However, the ratio improvement gradually slows down and eventually stops as the model goes deeper: when the model is deeper enough, it is able to cover all graphs in the layout dataset. The results on regular dataset as shown in Figure ?? also align with our proof. With the increase of the model depth, our method becomes more powerful regardless of what the aggregation function is. The phenomenon also demonstrates the theorem in (Loukas 2019), i.e., the product of the GNN’s depth and width must exceed a polynomial of the graph size to obtain an optimal result.

**Injective function** In Property 3, we demonstrate that an injective aggregation and combination function guarantee a more powerful AC-GNN. In our proposed GDN, we use summation as the aggregation function since sum aggregators can represent injective function over multisets (Lemma 5, (Xu et al. 2018a)). Here, we replace summation with mean aggregator to see its performance in the regular dataset. The results are shown in Figure ??, we can see that our method with sum aggregator is always better than the mean aggregator among all depths.

**Integrated AC-GNN & Equivalent nodes** In Property 1 and Property 2, we state the drawbacks of integrated scheme and equivalent nodes in the coloring problem. To solve these issues, we respectively summarize two rules to make AC-GNN more powerful: Do not use integrated AC-GNN and avoid equivalent nodes by assigning nodes different at-

<sup>3</sup><https://mat.tepper.cmu.edu/COLOR02/>

<sup>4</sup>[https://developers.google.com/optimization/cp/cp\\\_solver](https://developers.google.com/optimization/cp/cp\_solver)

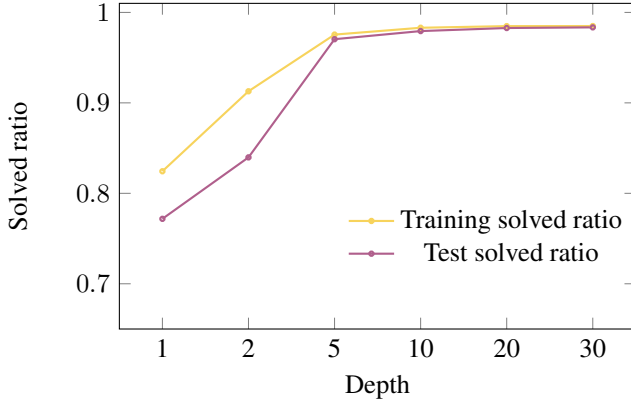

Figure 3: Comparison with different model depths on layout dataset.

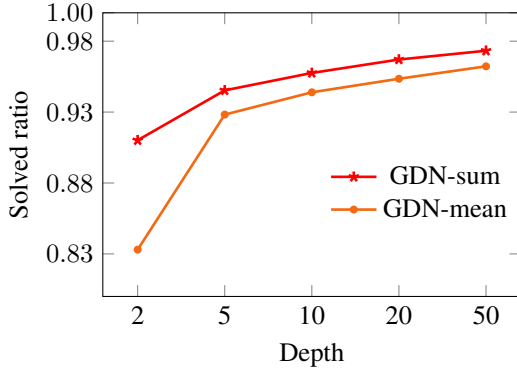

Figure 4: Comparison with mean aggregation on layout dataset.

tributes. We also try two variations of our methods, where the first one integrates the aggregation and combination:

$$\mathbf{h}_v^{(i)} = \lambda_C^{(i)} (\mathbf{h}_v^{(i-1)} + \sum_{u \in \mathcal{N}(v)} \mathbf{h}_u^{(i-1)}) + \beta^{(i)} \mathbf{1} \quad (17)$$

The second one set the node attribute as the same one while keep other steps the same. However, both variations fail to discriminate any two nodes, resulting in a zero solved ratio on all datasets after several layers.

### Other discussion.

**Postprocess.** We discuss the influence of our proposed GPU-friendly postprocess on the result quality and runtime. We compare our method with postprocess and without postprocess on layout dataset (Table 1) and normal dataset (Table 2). In the layout dataset, the relatively simple one, our post process can reduce the average predicted  $k$  by 1%. More importantly, the postprocess part makes our method optimal for more than 99.9% layout graphs except for the huge one, which occupies less than 0.1% in the total dataset. In the harder normal dataset, the conflict will increase by

Table 1: The results of our methods without postprocess and with concatenation on the layout dataset.  $k$  is the average predicted chromatic number, and the  $\uparrow$  (%) is the increase compared with Our original model.

|           |                | Small  | Med.   | Large  | Huge   |
|-----------|----------------|--------|--------|--------|--------|
| ILP       | $k$            | 3.0505 | 3.0151 | 3.0425 | 3.0612 |
| Ours      | $k$            | 3.0505 | 3.0151 | 3.0425 | 3.0645 |
| Ours      | $k$            | 3.0548 | 3.0181 | 3.0451 | 3.0669 |
| w.o. post | $\uparrow$ (%) | 1.4    | 1.0    | 0.9    | 0.8    |
| Ours      | $k$            | 3.0512 | 3.0151 | 3.0425 | 3.0653 |
| w. concat | $\uparrow$ (%) | 0.3    | 0      | 0      | 0.3    |

73.4% if postprocess is not used, as a scarifies, the runtime is increased by 12.8% when using postprocess. However, compared with the significant accuracy improvement, the time loss is acceptable, especially under the occasion that our method is  $500\times$  faster than a heuristic algorithm with a similar-quality. In Table 2, our method without postprocess sometimes even results in a better solution than the one with postprocess, this happens because we randomly initialize our node attribute, resulting in a slightly different solution everytime. Actually, we can further improve our performance by a repeated running like previous coloring methods (Zhou, Hao, and Duval 2016; Braunstein et al. 2006; Takefuji and Lee 1991), but our target is to provide insights for powerful GNNs on coloring problems instead of developing a powerful coloring solver by some simple tricks.

**Other techniques for heterophily.** In (Zhu et al. 2020b), they propose a concatenation technique for tasks under heterophily, i.e., concatenate all features in the middle layers, and compute the final embedding using the concatenated result. We also implement it for comparison, the results are shown in Table 1. According to the table, we can see that it fails to be effective in the coloring problem, which even increases  $k$  a little bit. Nevertheless, it is still an open and interesting question to find the effective techniques in the coloring tasks, and even in the general tasks under heterophily.

### References

- Abu-El-Haija, S.; Perozzi, B.; Kapoor, A.; Alipourfard, N.; Lerman, K.; Harutyunyan, H.; Steeg, G. V.; and Galstyan, A. 2019. Mixhop: Higher-order graph convolutional architectures via sparsified neighborhood mixing. *arXiv preprint arXiv:1905.00067*.
- Achlioptas, D.; and Naor, A. 2004. The two possible values of the chromatic number of a random graph. In *ACM Symposium on Theory of computing (STOC)*, 587–593.
- Barceló, P.; Kostylev, E. V.; Monet, M.; Pérez, J.; Reutter, J.; and Silva, J. P. 2019. The logical expressiveness of graph neural networks. In *International Conference on Learning Representations (ICLR)*.
- Braunstein, A.; Mézard, M.; Weigt, M.; and Zecchina, R. 2006. Constraint Satisfaction by Survey Propagation.
- Chen, Z.; Villar, S.; Chen, L.; and Bruna, J. 2019. On the equivalence between graph isomorphism testing

Table 2: The results of our method without postprocess on the normal dataset.

|                | Ours  |       | Ours w.o. post |       |
|----------------|-------|-------|----------------|-------|
|                | cost  | time  | cost           | time  |
| jean           | 0     | 0.13  | 0              | 0.11  |
| anna           | 0     | 0.17  | 0              | 0.15  |
| huck           | 0     | 0.13  | 5              | 0.11  |
| david          | 1     | 0.19  | 0              | 0.17  |
| homer          | 1     | 0.29  | 1              | 0.26  |
| myciel5        | 0     | 0.12  | 0              | 0.10  |
| myciel6        | 0     | 0.21  | 1              | 0.18  |
| games120       | 0     | 0.08  | 0              | 0.07  |
| Mug88_1        | 0     | 0.01  | 0              | 0.01  |
| 1-Insertions_4 | 0     | 0.07  | 0              | 0.07  |
| 2-Insertions_4 | 2     | 0.08  | 1              | 0.07  |
| Queen5_5       | 0     | 0.05  | 7              | 0.04  |
| Queen6_6       | 4     | 0.05  | 5              | 0.04  |
| Queen7_7       | 11    | 0.06  | 15             | 0.05  |
| Queen8_8       | 7     | 0.06  | 16             | 0.05  |
| Queen9_9       | 10    | 0.09  | 18             | 0.06  |
| Queen8_12      | 7     | 0.09  | 14             | 0.08  |
| Queen11_11     | 24    | 0.07  | 38             | 0.07  |
| Queen13_13     | 42    | 0.08  | 68             | 0.08  |
| ratio          | 1.000 | 1.000 | 1.734          | 0.872 |

and function approximation with gnns. *arXiv preprint arXiv:1905.12560*.

Dai, H.; Dai, B.; and Song, L. 2016. Discriminative embeddings of latent variable models for structured data. In *International conference on machine learning*, 2702–2711. PMLR.

Dai, H.; Khalil, E. B.; Zhang, Y.; Dilkina, B.; and Song, L. 2017. Learning combinatorial optimization algorithms over graphs. *arXiv preprint arXiv:1704.01665*.

Dasoulas, G.; Santos, L. D.; Scaman, K.; and Virmaux, A. 2019. Coloring graph neural networks for node disambiguation. *arXiv preprint arXiv:1912.06058*.

Defferrard, M.; Bresson, X.; and Vandergheynst, P. 2016. Convolutional neural networks on graphs with fast localized spectral filtering. *arXiv preprint arXiv:1606.09375*.

Gamarnik, D.; and Sudan, M. 2014. Limits of local algorithms over sparse random graphs. In *Proceedings on Innovations in theoretical computer science*, 369–376.

Gualandi, S.; and Malucelli, F. 2012. Exact solution of graph coloring problems via constraint programming and column generation. *INFORMS Journal on Computing*, 24(1): 81–100.

Hagberg, A. A.; Schult, D. A.; and Swart, P. J. 2008. Exploring Network Structure, Dynamics, and Function using NetworkX. In Varoquaux, G.; Vaught, T.; and Millman, J., eds., *Proceedings of the 7th Python in Science Conference*, 11 – 15. Pasadena, CA USA.

Hamilton, W.; Ying, Z.; and Leskovec, J. 2017. Inductive representation learning on large graphs. In *Annual Con-*

*ference on Neural Information Processing Systems (NIPS)*, 1024–1034.

Holme, P.; and Kim, B. J. 2002. Growing scale-free networks with tunable clustering. *Physical review E*, 65(2): 026107.

Huang, J.; Patwary, M.; and Damos, G. 2019. Coloring big graphs with alphagozero. *arXiv preprint arXiv:1902.10162*.

Jiang, I. H.-R.; and Chang, H.-Y. 2017. Multiple patterning layout decomposition considering complex coloring rules and density balancing. *IEEE Transactions on Computer-Aided Design of Integrated Circuits and Systems (TCAD)*, 36(12): 2080–2092.

Kingma, D. P.; and Ba, J. 2014. Adam: A method for stochastic optimization. *arXiv preprint arXiv:1412.6980*.

Lemos, H.; Prates, M.; Avelar, P.; and Lamb, L. 2019. Graph colouring meets deep learning: Effective graph neural network models for combinatorial problems. In *IEEE International Conference on Tools with Artificial Intelligence (IC-TAI)*, 879–885. IEEE.

Li, P.; Wang, Y.; Wang, H.; and Leskovec, J. 2020a. Distance Encoding–Design Provably More Powerful GNNs for Structural Representation Learning. *Annual Conference on Neural Information Processing Systems (NeurIPS)*.

Li, W.; Ma, Y.; Sun, Q.; Lin, Y.; Jiang, I. H.-R.; Yu, B.; and Pan, D. Z. 2019. OpenMPL: An Open Source Layout Decomposer. In *2019 IEEE 13th International Conference on ASIC (ASICON)*, 1–4. IEEE.

Li, W.; Xia, J.; Ma, Y.; Li, J.; Liny, Y.; and Yu, B. 2020b. Adaptive Layout Decomposition with Graph Embedding Neural Networks. In *2020 57th ACM/IEEE Design Automation Conference (DAC)*, 1–6. IEEE.

Li, Z.; Chen, Q.; and Koltun, V. 2018. Combinatorial optimization with graph convolutional networks and guided tree search. In *Annual Conference on Neural Information Processing Systems (NIPS)*, 539–548.

Lou, Z.; You, J.; Wen, C.; Canedo, A.; Leskovec, J.; et al. 2020. Neural Subgraph Matching. *arXiv preprint arXiv:2007.03092*.

Loukas, A. 2019. What graph neural networks cannot learn: depth vs width. *arXiv preprint arXiv:1907.03199*.

Maron, H.; Ben-Hamu, H.; Serviansky, H.; and Lipman, Y. 2019. Provably powerful graph networks. *arXiv preprint arXiv:1905.11136*.

Maron, H.; Ben-Hamu, H.; Shamir, N.; and Lipman, Y. 2018. Invariant and equivariant graph networks. *arXiv preprint arXiv:1812.09902*.

Morris, C.; Ritzert, M.; Fey, M.; Hamilton, W. L.; Lenssen, J. E.; Rattan, G.; and Grohe, M. 2019. Weisfeiler and leman go neural: Higher-order graph neural networks. In *AAAI Conference on Artificial Intelligence*, volume 33, 4602–4609.

OPTIMIZATION, G. 2014. INC. Gurobi optimizer reference manual, 2015. URL: <http://www.gurobi.com>, 29.

Pei, H.; Wei, B.; Chang, K. C.-C.; Lei, Y.; and Yang, B. 2020. Geom-GCN: Geometric graph convolutional networks. *arXiv preprint arXiv:2002.05287*.

- Rahman, M.; Virag, B.; et al. 2017. Local algorithms for independent sets are half-optimal. *The Annals of Probability*, 45(3): 1543–1577.
- Sato, R.; Yamada, M.; and Kashima, H. 2019. Approximation ratios of graph neural networks for combinatorial problems. *arXiv preprint arXiv:1905.10261*.
- Sato, R.; Yamada, M.; and Kashima, H. 2020. Random Features Strengthen Graph Neural Networks. *arXiv preprint arXiv:2002.03155*.
- Sen, P.; Namata, G.; Bilgic, M.; Getoor, L.; Galligher, B.; and Eliassi-Rad, T. 2008. Collective classification in network data. *AI magazine*, 29(3): 93–93.
- Takefuji, Y.; and Lee, K. C. 1991. Artificial neural networks for four-coloring map problems and K-colorability problems. *IEEE Transactions on Circuits and Systems I*, 38(3): 326–333.
- Wang, M.; Yu, L.; Zheng, D.; Gan, Q.; Gai, Y.; Ye, Z.; Li, M.; Zhou, J.; Huang, Q.; Ma, C.; et al. 2019. Deep graph library: Towards efficient and scalable deep learning on graphs. *arXiv preprint arXiv:1909.01315*.
- Watts, D. J.; and Strogatz, S. H. 1998. Collective dynamics of ‘small-world’ networks. *nature*, 393(6684): 440–442.
- Weisfeiler, B.; and Lehman, A. A. 1968. A reduction of a graph to a canonical form and an algebra arising during this reduction. *Nauchno-Tekhnicheskaya Informatsia*, 2(9): 12–16.
- Wu, Q.; and Hao, J.-K. 2012. Coloring large graphs based on independent set extraction. *Computers & Operations Research*, 39(2): 283–290.
- Xu, K.; Hu, W.; Leskovec, J.; and Jegelka, S. 2018a. How powerful are graph neural networks? *arXiv preprint arXiv:1810.00826*.
- Xu, K.; Li, C.; Tian, Y.; Sonobe, T.; Kawarabayashi, K.-i.; and Jegelka, S. 2018b. Representation learning on graphs with jumping knowledge networks. In *International Conference on Machine Learning*, 5453–5462. PMLR.
- Xu, K.; Li, J.; Zhang, M.; Du, S. S.; Kawarabayashi, K.-i.; and Jegelka, S. 2019. What can neural networks reason about? *arXiv preprint arXiv:1905.13211*.
- You, J.; Gomes-Selman, J.; Ying, R.; and Leskovec, J. 2021. Identity-aware Graph Neural Networks. *arXiv preprint arXiv:2101.10320*.
- You, J.; Ying, R.; and Leskovec, J. 2019. Position-aware graph neural networks. *arXiv preprint arXiv:1906.04817*.
- You, J.; Ying, R.; and Leskovec, J. 2020. Design space for graph neural networks. *arXiv preprint arXiv:2011.08843*.
- Yu, B.; Yuan, K.; Ding, D.; and Pan, D. Z. 2015. Layout decomposition for triple patterning lithography. *IEEE Transactions on Computer-Aided Design of Integrated Circuits and Systems*, 34(3): 433–446.
- Zhou, Y.; Hao, J.-K.; and Duval, B. 2016. Reinforcement learning based local search for grouping problems: A case study on graph coloring. *Expert Systems with Applications*, 64: 412–422.
- Zhu, J.; Rossi, R. A.; Rao, A.; Mai, T.; Lipka, N.; Ahmed, N. K.; and Koutra, D. 2020a. Graph Neural Networks with Heterophily. *arXiv preprint arXiv:2009.13566*.
- Zhu, J.; Yan, Y.; Zhao, L.; Heimann, M.; Akoglu, L.; and Koutra, D. 2020b. Beyond Homophily in Graph Neural Networks: Current Limitations and Effective Designs. *Advances in Neural Information Processing Systems*, 33.
