# Supplementary material for: Rethinking Graph Neural Networks for the Graph Coloring Problem
Source: arXiv:2208.06975 source file (2022-08-19)
Supplement: Supplementary file 3 [file setting-cv.tex]

% =============================================================
%         Setting for CV papers
%
%   Author      : Bei Yu
%   Last Update : 04/2018
% =============================================================

% === comment out for ICCV
%\makeatletter
%\@namedef{ver@everyshi.sty}{}
%\makeatother

\usepackage{times}
\usepackage{epsfig}
\usepackage{graphicx}
\usepackage{amsmath,amsfonts,amssymb,amsthm}
\usepackage{subfig}
\captionsetup[subfigure]{labelformat=simple}               % avoid "double brackets" in sub-figure caption
             % "Fig.~1b"-->"Fig.1(b)"
%\usepackage[colorlinks]{hyperref}
\usepackage[pagebackref=true,breaklinks=true,letterpaper=true,colorlinks,bookmarks=false]{hyperref}
\hypersetup{
    pageanchor=false,
    linkcolor=blue,
    anchorcolor=blue,
    citecolor=blue,
    urlcolor=blue,
    plainpages=false,
}
\usepackage{cleveref}
\usepackage{caption}
\usepackage{algpseudocode}                                 % new algorithm package
\usepackage{algorithm}
       % Use Input in the format of Algorithm
       % Use Output in the format of Algorithm
\usepackage{tikz}
\usepackage{pgfplots}
\usepackage{pgfplotstable}
\pgfplotsset{compat=newest}
\usepackage{filecontents}
\usepackage{booktabs}             % professional-quality tables
\usepackage{tabularx}
\usepackage{multirow}
\usepackage{color}
\usepackage[flushleft]{threeparttable}
\usepackage{bm}
\usepackage{textcomp}             % for degree symbol
\usepackage{enumitem}

% ==== Local new commands

    % re-define vec command

% ==== Theorem Definitions
