# Supplementary material for: Rethinking Graph Neural Networks for the Graph Coloring Problem
Source: arXiv:2208.06975 source file (2022-08-19)
Supplement: Supplementary file 4 [file appendix.tex]

\providecommand{\customgenericname}{}
\newcommand{\newcustomtheorem}[2]{%
  \newenvironment{#1}[1]
  {%
   \renewcommand\customgenericname{#2}%
   \renewcommand\theinnercustomgeneric{##1}%
   \innercustomgeneric
  }
  {\endinnercustomgeneric}
}

\newcustomtheorem{customprop}{Proposition}
\newcustomtheorem{customthem}{Theorem}
\newcustomtheorem{customcorollary}{Corollary}
\appendix

\section{Graph Terminology}
\label{appendix:term}
Here we list the following graph theoretic terms encountered in our work:

\paragraph{Basic graph teminology.}
Let $\gG = (\gV,\gE)$ and $\gG' = (\gV',\gE')$ be graphs on vertex set $\gV$ and $\gV'$, we define
\begin{itemize}[leftmargin=*]
    \item \textit{isomorphism}: we say that a bijection $\pi: \gV \rightarrow \gV'$ is an \textit{isomorphism} if any two vertices $u,v \in \gV$ are adjacent in $\gG$
    if and only if $\pi(u),\pi(v) \in \gV'$ are adjacent in $\gG'$, i.e., $\{u,v\} \in \gE $ iff $\{\pi(u),\pi(v)\} \in \gE' $.
    \item \textit{isomorphic nodes}: If there exists the isomorphism between $\gG$ and $\gG'$, we say that $\gG$ and $\gG'$ are \textit{isomorphic}.
    \item \textit{automorphism}: When $\pi$ is an isomorphism of a vertex set onto itself, i.e., $\gV = \gV'$,
    $\pi$ is called an \textit{automorphism} of $\gG$.
    \item \textit{topologically equivalent}: We say that the node pair $\{u,v\}$ is \textit{topologically equivalent} if there is an automorphism mapping one to the other, i.e., $v = \pi(u)$.
    \item \textit{equivalent}: $\{u,v\}$ is \textit{equivalent} if it is topologically equivalent by $\pi$ and $\vx_w = \vx_{\pi(w)}$ holds for every $w \in \gV$,
    where $\vx_w$ is the node attribute of node $w$.
    \item \textit{$r$-local automorphism}:
    A bijection $\pi_r: \gV \rightarrow \gV$ is an \textit{$r$-local automorphism} that maps $u$ to $v$ if $\pi_r$ is an isomorphism from $\gB_{\gG}(u,r)$ to $\gB_{\gG}(v,r)$.
    \item \textit{$r$-local topologically equivalent}: the node pair $\{u,v\}$ is \textit{$r$-local topologically equivalent}
    if $\pi_r$ is an isomorphism from $\gB_{\gG}(u,r)$ to $\gB_{\gG}(v,r)$.
\end{itemize}

\section{Proofs}
\subsection{Proof of Proposition \ref{nonoptACGNN}}
We first recall the proposition.
    \begin{customprop}{1}
    All AC-GNNs cannot discriminate any equivalent node pair.
    \end{customprop}
    \begin{proof}
    Let $\pi$ be the automorphism mapping $u$ to $v$, here, we propose a stronger proposition:

    \begin{myprop}
        \label{nonoptACGNN2}
    Given an AC-GNN and an equivalent node pair $\{u,v\}$ by $\pi$, $\vh_w^i = \vh_{\pi(w)}^i $ holds for any iteration $i$ and any node $w \in \gV$.
    \end{myprop}

    This apparently holds for $i=0$ since $\vx_w = \vx_{\pi(w)}, \forall w \in \gV$.
    Suppose this holds for iteration $j$, i.e., $\vh_w^j = \vh_{\pi(w)}^j, \forall w \in \gV$.
    By definition, AC-GNN $\gA$ produces the feature vector $\vh_v^{j+1}$ of node $v$ in the $(j+1)_{th}$ iteration as follows:
    \begin{align}
        \vh_v^{(j+1)} = \text{COM}^{(j+1)}(\vh_v^{(j)}, \text{AGG}^{(j+1)}(\{\vh_u^{(j)}:u\in \gN(v) \})).
       \end{align}

    Since an automorphism $\pi$ remains the set of edges, i.e., $\{u,v\} \in \gE$ iff $\{\pi(u),\pi(v)\} \in \gE$,
    the connection relation between two neighbors is preserved after the permutation by $\pi$, that is, $\gN(\pi(v)) = \{\pi(u), u \in \gN(v)\}$ for any $v \in \gV$.
    Then, the input of $\text{AGG}^{(j+1)}$ for $\pi(v)$ is given by $\{\vh_{u}^{(j)}:u\in \gN({\pi(v)}) \}$,
    which is $\{\vh_{\pi(u)}^{(j)}:u\in \gN({v}) \}$. Since $\vh_w^j = \vh_{\pi(w)}^j, \forall w \in \gV$,
    the input of $\text{AGG}^{(j+1)}$ for $v$ is equal to the one of $\text{AGG}^{(j+1)}$ for ${v}$, i.e., $\{\vh_{\pi(u)}^{(j)}:u\in \gN({v}) \} = \{\vh_{\pi(u)}^{(j)}:u\in \gN({v}) \}$
    and makes their output equal, i.e., $\vm_{v}^{j+1} = \vm_{\pi(v)}^{j+1}$. Therefore, the input of COM$^{(j+1)}$ for $v$, $(\vh_v^{(j)}, \vm_{v}^{j+1})$, is also equal to the one of COM$^{(j+1)}$ for $\pi(v)$,
    which makes the vector features of $v$ and $\pi(v)$ equal after $(j+1)_{th}$ iteration for any node $v \in \gV$ and proves the proposition \ref{nonoptACGNN2}.
    Thus, the AC-GNN $\gA$ always produces the same node embeddings for the nodes in the equivalent node pair, which results in the same color.

\end{proof}

\subsection{Proof of Proposition \ref{nonoptHACGNN}}
We first recall the proposition.
    \begin{customprop}{2}
    There is a graph in which at least one distinct node pair is not discriminated by any integrated AC-GNN.
    \end{customprop}

    \begin{proof}
    The proof starts with a simple fact: a classifier $CLS(\cdot)$ always assign two nodes with the same node embedding to the same category.

    Consider the following graph $\gG = (\gV,\gE)$, in which two connected nodes $u$ and $v$ share the same neighborhood except each other,
    i.e., $\gN(u) \backslash \{v\} = \gN(v)\backslash \{u\}$. The node pair $\{u,v\}$ is distinct since they are connected.
    % The node features of $u$ after $k$ iterations, $\vh_u^k$, is calculated by:
    % \begin{align}
    %     \vh_u^{(j)} = \text{COM}^{(j)}(\text{AGG}(\{\vh_w^{(k-1)}:w\in \gN(u) \cup \{u\}\})).
    %    \end{align}
    % Similarly, $\vh_v^k$ is calculated by:
    % \begin{align}
    %     \vh_v^{(j)} = \text{COM}^{(j)}(\text{AGG}(\{\vh_w^{(k-1)}:w\in \gN(v) \cup \{v\}\})).
    %    \end{align}
       It follows that the inputs for the node features of $u$ and $v$ after iteration $k$ are exactly the same since
       $\gN(u) \cup \{u\}= \gN(u)\backslash \{v\} \cup \{u,v\} =\gN(v)\backslash \{u\} \cup \{u,v\} = \gN(v) \cup \{v\}$.
       Therefore, the outputs are the same, which means that $\vh_u^{(j)} = \vh_v^{(j)}$ holds for any iteration $k$ and any aggregation and combine functions $\text{AGG}(\cdot),\text{COM}(\cdot)$.
       Combining with the fact that $CLS(\vh_u) =CLS(\vh_v)$ if $\vh_u = \vh_v$, the proof is finished.
    \end{proof}

    \subsection{Proof of Corollary \ref{nonoptlocal}}
    We first recall the corollary.
    \begin{customcorollary}{1}
            A local coloring method is non-optimal in the random d-regular graph as $d\rightarrow \infty$.
    \end{customcorollary}
    \begin{proof}
        A random $d$-regular graph $\gG_d^n$ is a graph with $n$ nodes and each node pair is connected with a probability $d/n$.
        We start the proof from the following non-trivial proposition:
        \begin{myprop}[\cite{rahman2017local}]
            \label{halfMIS}
            The largest density of factor of i.i.d. independent sets in a random d-regular graph is asymptotically at most $(\log d)/d$ as $d\rightarrow \infty$.
            The density of the largest independent sets in these graphs is asymptotically $2(\log d)/d$.
        \end{myprop}
        The proposition above limits the size of an independent set produced by a local method for the random $d$-regular graph with an upper bound, $n(\log d)/d$ as $d\rightarrow \infty$.
        Given an upper bound of the independent set, the following corollary on the graph coloring problem is introduced:
        \begin{customcorollary}{2}
            \label{k_lb}
            The lower bound of k with a zero conflict constraint obtained by a local coloring method for the random $d$-regular graph is $d/\log d$ as $d\rightarrow \infty$.
        \end{customcorollary}
        The proof is based on the Proposition \ref{halfMIS}: if a local coloring method $f$ obtains a smaller $k'$, s.t. $k'< d/\log d$ by coloring $\gG_d^n$ without conflict using $k'$ colors,
        all node sets classified by the node color will be independent sets and the size of the maximum one will be larger than $(n\log d)/d$, a contradiction with Proposition \ref{halfMIS}.

        The Corollary \ref{k_lb} reveals the lower bound of $k$ by local methods for a random $d$-regular graph.
        Another important observation of $k$ by \cite{achlioptas2004two} specifies that exact value of the chromatic number (i.e., the minimum $k$) of a random $d$-regular graph.
        The proposition is described as follows:
        \begin{myprop}[\cite{achlioptas2004two}]
            \label{local_k}
            Let $t_d$ be the smallest integer $t$ such that $d < 2t \log t$. The chromatic number of a random $d$-regular graph is either $t_d$ or $t_d + 1$.
        \end{myprop}

        It follows directly from Corollary \ref{k_lb} and Proposition \ref{local_k} that,
        we can finish the proof of Corollary \ref{nonoptlocal} by showing that the lower bound of $k$ by local methods is always greater than the exact chromatic number:
        \begin{equation}
            d/\log d > t_d + 1 \ \text{for } \ d \rightarrow \infty.
           \end{equation}

        Let $f(t) = 2t\log t$ and define $t_0$ s.t. $d = f(t_0) = 2t_0 \log t_0$.
        Since $t_d$ is the smallest integer $t$ such that $d < f(t)$, we have $f(t_0) = d \geq f(t_d -1) $.
        Since $f$ is monotonically increasing, $t_0 \geq t_d - 1$ and thus $d/\log d - t_d -1 \geq d/\log d - t_0 -2$ always holds.
        % Let $h(d) = d/\log d - f^{-1}(d) -2$, the inequality above is transformed to:
        % \begin{equation}
        %     h(d)= d/\log d - f^{-1}(d) -2 > 0 \ \text{for } \ d \rightarrow \infty.
        % \end{equation}
        Let $d = 2t_0 \log t_0 $, we further derive the objective below:
        \begin{align*}
            &d/\log d - t_d -1 \geq d/\log d - t_0 -2  \\ 
            =& \frac{2 t_0\log t_0}{\log(2t_0 \log t_0)}-t_0-2 > 0, \ \text{for } \ d,t_0 \rightarrow \infty.
        \end{align*}
        we first prove that
        \begin{align*}
            &\frac{\log t_0}{\log(2t_0 \log t_0)}>2/3\\
            \Rightarrow&3\log t_0>2\log(2t_0\log t_0)\\
            \Rightarrow&3\log t_0>2(1+\log t_0+\log (\log t_0))\\
            \Rightarrow&\log t_0>2+2\log(\log t_0) \ \text{ when } t_0\to \infty.
        \end{align*}
        The above inequality holds obviously.
        Following the objective, we have:

        \begin{align*}
            &\frac{2 t_0\log t_0}{\log(2t_0 \log t_0)}-t_0-2  
            \\> &\frac{4}{3}t_0-t_0-2 >0  \ \text{ when } t_0\to \infty.
        \end{align*}
        Therefore, we finish the proof.
        %    Consider $f(x)=2x\log x.$ This f(x) has inverse function $f_1(x)=y=e^{\frac{x}{2y}}.$ 

        %    Differentiate the $f_1$, we have $$\frac{dy}{dx}=\frac{y}{2y+x}.$$ 
           
        %    Note that $h(x)$ is nothing but $h(x)=\frac{x}{\log x}-y-2.$ 
           
        %    Not hard to find a $x_1$ s.t. $h(x_1)>0.$
           
        %    Differentiate $h(x)$, we have $$h'(x)=(\frac{x}{\log x})'-\frac{dy}{dx}=()\ln 2)(\frac{\log x -1}{\log^2 x}-\frac{y}{2y+x}).$$
           
        %    Note that by $y=e^{\frac{x}{2y}}$, which is equivalent to $x=2y\log y$, we note that as $x \to \infty$, $y \to \infty.$
           
        %    Rewrite $h'(x)$ into a form with only $y$, we have $$h'(x)=\frac{\log(2y\log y)-1}{[\log(2y\log y)]^2}-\frac{y}{2y+2y\log y}.$$ 
           
        %    Let $\log y =a$ Note that $h'(x) \geq 0$ is equivalent to $$(a+\log 2a)^2 \geq 2(\log 2a)^2 +2,$$ iff, $$(\frac{a}{\log 2a}+1)^2 \geq 2+ \frac{2}{(\log 2a)^2},$$ iff, $$\frac{a^2}{(\log 2a)^2}+\frac{2a}{\log 2a}\geq 1+\frac{2}{(\log 2a)^2},$$ iff, $$\frac{a^2-2}{(\log 2a)^2}+\frac{2a}{\log 2a}-1\geq 0$$
           
        %    Suffice to choose $a$ s.t. $a>a_1$. 
           
        %    (Because $\forall x \geq 0, x \geq \log(x+1)$, which is, $\frac{x}{\log (x+1)} \geq 1$.)
           
        %    So, such $a_0$ can be found, which implies such $y_0$ can be found, because $a_0=\log y_0$, and also, then such $x_0$ can be found, because $x_0=2y_0\log y_0.$
        
        %    This means that $\forall x>x_0, h'(x)\geq 0.$ Not hard to find a $x_1>x_0.$
        \end{proof}

    \subsection{Proof of Corollary \ref{prop:local}}
    We first recall the corollary.

    \begin{customcorollary}{2}
        AC-GNN is a local coloring method.
    \end{customcorollary}
    \begin{proof}
        Given an AC-GNN $\gA$ with $L$ layers,
        let's consider a $L$-local equivalent node pair $\{u,v\}$ in $\gG$ by an $L$-local automorphism $\pi_L$,
        which means that two rooted subtrees $\gB_\gG(u,L)$ and $\gB_\gG(v,L)$ are isomorphic and $\vx_w = \vx_{\pi_r(w)}$ holds for every $w \in \gB_{\gG}(u,r)$.
        Since two rooted subtrees are isomorphic,
        the WL test \cite{weisfeiler1968reduction} decides $\gB_\gG(u,L)$ and $\gB_\gG(v,L)$ are isomorphic
        and assigns the same color to $w$ and $\pi_L(w)$ for any $w \in \gB_\gG(u,L)$.
        To connect the WL test with AC-GNN, the following proposition is used:
        \begin{myprop}[\cite{morris2019weisfeiler,barcelo2019logical,xu2018powerful}]
            \label{nonoptACGNN1}
        If the WL test assigns the same color to two nodes in a graph, then every AC-GNN maps the two nodes into the same node embedding.
        \end{myprop}
        Therefore, $\gA$ maps the $u$ and $v$ into the same node embedding.
        It follows that $\gA$ is $L$-local and thus local.
    \end{proof}

    \subsection{Proof of Theorem \ref{colorequa}}
    We first recall the theorem.
    \begin{customthem}{2}
        Let $\gA$ be a simple AC-GNN and both input and output of each layer in $\gA$ be the probability distribution $\vh \in \R^{k}$ of $k$ colors,
        $\gA$ is color equivariant if and only if the following conditions hold:
        \begin{itemize}
            \item For any layer $i$, all the off-diagonal elements of $\mC^{(i)}$ are tied together and all the diagonal elements are equal as well. That is,
        \begin{align}
            &\mC^{(i)} =  \lambda_C^{(i)}\mI + \gamma_C^{(i)}(\text{\textbf{11}}^{\top}) \nonumber \\
              & \lambda_C^{(i)},\gamma_C^{(i)} \in \R \ \  ;  \textbf{1} = [1,...,1]^{\top} \in \R^k.
           \end{align}

            \item For any layer $i$, all the off-diagonal elements of $\mA^{(i)}$ are also tied together and all the diagonal elements are equal as well. That is,
            \begin{align}
                &\mA^{(i)} = \lambda_A^{(i)}\mI + \gamma_A^{(i)}(\text{\textbf{11}}^{\top}) \nonumber \\ &  \lambda_A^{(i)},\gamma_A^{(i)} \in \R \ \ \textbf{1} = [1,...,1]^{\top} \in \R^k.
               \end{align}
            \item For any layer $i$, all elements in $\vb^{(i)}$ are equal. That is,
            \begin{equation}
                \vb^{(i)} = \beta^{(i)}\text{\textbf{1}} \ \ \  \beta^{(i)} \in \R \ \ \textbf{1} = [1,...,1]^{\top} \in \R^k.
               \end{equation}
        \end{itemize}
    \end{customthem}

    \begin{proof}
        Let AGG$^{(i)}$ and COM$^{(i)}$ be the aggregation and combination functions in the $i_{th}$ layer of $\gA$.
        $\gA$ is color equivariant if and only if all functions in $\{\text{AGG}^{(i)},\text{COM}^{(i)}: i\in {1,...,L}\}$ are color equivariant.
        the aggregation function is color equivariant clearly and thus we are left to consider the color equivariance of combination functions.
        Considering the definition of color equivariant in Definition \ref{def:color_eq},
        the color equivariance of combination function COM$^{(i)} = \sigma (\vx\mC^{(i)} + \vy\mA^{(i)}+\vb^{(i)})$ is given by:
        \begin{equation}
            \label{color_equivariance}
            \sigma (\vx\mC^{(i)} + \vy\mA^{(i)}+\vb^{(i)})\mP  = \sigma (\vx\mP \mC^{(i)} + \vy\mP \mA^{(i)}+\vb^{(i)}).
        \end{equation}
        COM$^{(i)}$ is color equivariant if and only if the equation above holds for any permutation matrix $\mP \in \R^{k\times k}$ and any vectors $\vx,\vy$.
        Considering it holds for any vectors $\vx,\vy$, We first find three special cases of $\vx$ and $\vy$, which are necessary conditions and correspond to three conditions respectively:

        \textit{Case 0}. When $\vy = \vec{0}$, we have that $\sigma(\vx \mC^{(i)}) \mP = \sigma(\vx \mP \mC^{(i)})$ holds for any $\mP$ and $\vx$.
        That is, $\vx(\mC^{(i)}\mP - \mP \mC^{(i)}) = \vec{0} $ always holds, which reveals that $\mC^{(i)}\mP = \mP \mC^{(i)}$.
        $\mC^{(i)}\mP = \mP \mC^{(i)}$ holds for any $\mP$ follows that $\emC^{(i)}_{m,m} = \emC^{(i)}_{n,n}$ and $\emC^{(i)}_{m,n} = \emC^{(i)}_{n,m}$ for any $m,n \in \{1,...,k\}$.
        Therefore, all the off-diagonal elements of $\mC^{(i)}$ are tied together and all the diagonal elements are equal as well.

        \textit{Case 1}. When $\vx = \vec{0}$, we can prove that all the off-diagonal elements of $\mA^{(i)}$ are tied together and all the diagonal elements are equal as well following the similar induction in case 1.

        \textit{Case 2}. When $\vx = \vy = \vec{0}$, we have that $\sigma(\vb^{(i)}) \mP  = \sigma(\vb^{(i)})$ holds for any $\mP$. Therefore, all elements in $\vb^{(i)}$ are equal.

        After proving that these conditions are necessary for a color equivariant $\gA$, we proceed to prove that the conditions above are already sufficient.
        Let $\mC^{(i)} = \lambda_C^{(i)}\mI + \gamma_C^{(i)}(\text{\textbf{11}}^{\top})$, $\mA^{(i)} = \lambda_A^{(i)}\mI + \gamma_A^{(i)}(\text{\textbf{11}}^{\top})$ and $\vb^{(i)} =  \beta^{(i)}\text{\textbf{1}}$,
        COM$^{(i)}$ is then calculated by:
        \begin{align}
            \text{COM}^{(i)} \mP &=\sigma(\vx\mC^{(i)} + \vy\mA^{(i)}+\vb^{(i)})\mP \nonumber \\
             &=\sigma(\vx \lambda_C^{(i)}\mI \mP + \vx \gamma_C^{(i)}(\text{\textbf{11}}^{\top}) \mP+ \vy \lambda_A^{(i)}\mI\mP \nonumber
             \\ & + \vy \gamma_A^{(i)}(\text{\textbf{11}}^{\top})\mP +\beta^{(i)}\text{\textbf{1}} \mP) \nonumber \\
             &=\sigma(\vx \mP \lambda_C^{(i)}\mI + \vx \mP \gamma_C^{(i)}(\text{\textbf{11}}^{\top}) + \vy \mP \lambda_A^{(i)}\mI  \nonumber 
             \\ & + \vy \mP \gamma_A^{(i)}(\text{\textbf{11}}^{\top})+ \beta^{(i)}\text{\textbf{1}}) \nonumber \\
             &=\sigma (\vx\mP \mC^{(i)} + \vy\mP \mA^{(i)}+\vb^{(i)}).
        \end{align} 
        Therefore,  COM$^{(i)}$ is color equivariant if and only if the conditions hold, which completes the proof.

    \end{proof}

\begin{table*}[tb!]
    \centering
    \caption{Graph datasets information and time performance by different coloring methods on CPU.}
    \label{tab:dimacs}
    %\resizebox{0.96\linewidth}{!}{
    \begin{tabular}{llllll|l|l}
    \toprule
    \multirow{2}{*}{\textbf{Dataset}} &
      \multirow{2}{*}{\textbf{Graph}} &
      \multirow{2}{*}{\textbf{$|\gV|$}} &
      \multirow{2}{*}{\textbf{$|\gE|$}} &
      \multirow{2}{*}{\textbf{d\%}} &
      \multirow{2}{*}{\textbf{$\chi(k)$}} &
      \textbf{GNN-GCP} &
      \textbf{Ours} \\
                              &                 &        &        &      &    & Time    & Time   \\ \midrule
    Layout                    & 35158           & 641202 & 787242 & -    & 3  & 1724.62 & 355.73 \\ \midrule
    \multirow{3}{*}{Citation} & Cora            & 2708   & 5429   & 0.15 & 5  & 2.79    & 0.55   \\
                              & Citeseer        & 3327   & 4732   & 0.09 & 6  & 4.09    & 0.86   \\
                              & Pubmed          & 19717  & 44338  & 0.03 & 8  & 120.5   & 5.10   \\ \midrule
    \multirow{3}{*}{Random} &
      Power Law Tree &
      7956 &
      7756 &
      2.8 &
      - &
      4.08 &
      2.30 \\
                              & Small World     & 7956   & 29716  & 10.7 & -  & 3.04    & 6.05   \\
                              & Holme and Kim   & 7956   & 15712  & 5.7  & -  & 3.00    & 25.12  \\ \midrule
    \multirow{18}{*}{COLOR}   & jean            & 80     & 254    & 8    & 10 & 0.25    & 0.04   \\
                              & anna            & 138    & 493    & 5    & 11 & 0.04    & 0.04   \\
                              & huck            & 74     & 301    & 11   & 11 & 0.03    & 0.06   \\
                              & david           & 87     & 406    & 11   & 11 & 0.02    & 0.07   \\
                              & homer           & 561    & 1628   & 1    & 13 & 0.59    & 0.10   \\
                              & myciel5         & 47     & 236    & 22   & 2  & 0.02    & 0.03   \\
                              & myciel6         & 95     & 755    & 17   & 2  & 0.04    & 0.05   \\
                              & games120        & 120    & 638    & 9    & 9  & 0.04    & 0.03   \\
                              & Mug88\_1        & 88     & 146    & 4    & 3  & 0.03    & 0.01   \\
                              & 1-Insertions\_4 & 67     & 232    & 10   & 2  & 0.03    & 0.05   \\
                              & 2-Insertions\_4 & 212    & 1621   & 7    & 4  & 0.05    & 0.04   \\
                              & Queen5\_5       & 25     & 160    & 53   & 5  & 0.01    & 0.02   \\
                              & Queen6\_6       & 36     & 290    & 46   & 6  & 0.02    & 0.02   \\
                              & Queen7\_7       & 49     & 476    & 40   & 7  & 0.15    & 0.03   \\
                              & Queen8\_8       & 64     & 728    & 36   & 8  & 0.03    & 0.02   \\
                              & Queen9\_9       & 81     & 1056   & 33   & 9  & 0.04    & 0.07   \\
                              & Queen8\_12      & 96     & 1368   & 30   & 12 & 0.05    & 0.05   \\
                              & Queen11\_11     & 121    & 3960   & 55   & 11 & 0.06    & 0.07   \\
                              & Queen13\_13     & 169    & 6656   & 47   & 13 & 0.09    & 0.11   \\ \bottomrule
    \end{tabular}
    %}
\end{table*}

\section{Related Works}

\section{Preproces \& Postprocess}

\section{Global method}
\section{Supplementary Experiments}

Previously in Section 5, we conducted our experiments with GPU acceleration. For a more complete performance comparison between our model and the baselines, we conducted supplementary, CPU-only experiments on our model and other NN-based baselines, and recorded the running time as shown in the table below.
